# Supplementary material for: NumS: Scalable Array Programming for the Cloud
Source: arXiv:2206.14276 source file (2022-07-13)
Supplement: Supplementary file 1 [file 004-blocked-operations.tex]

\section{Parallel Blocked Matrix and Vector Operations}
\label{appendix:blocked}

In this section, we detail blocked matrix representations, their operations, and a generalization of these concepts to $n$ dimensions.

\subsection{Blocked Representations and Operations}

The {\it block} decomposition of vectors and matrices can be described as follows.  For a matrix $\X \in \mathbb{R}^{n_1 \times n_2}$, let $g_1$ and $g_2$ be the dimensions of the {\it grid} of blocks into which $\X$ is decomposed. For $i \in \{ 0, \dots, g_1-1\}$ and $j \in \{ 0, \dots, g_2-1\}$, let $\X_{i,j}$ denote the $i,j$ block of $\X$, as depicted in the following equation.
\begin{align}
\X & =
\begin{bmatrix}
    \X_{0, 0} & \dots & \X_{0, g_2-1}  \\
    \vdots & \ddots & \vdots \\
     \X_{g_1-1, 0} & \dots & \X_{g_1-1, g_2-1}
 \end{bmatrix}
 \label{eq:blocks}
\end{align}
Note that each block $\X_{i,j}$ {\it is itself a matrix with dimensions $(n_1/g_1) \times (n_2/g_2)$}. For brevity, we assume the dimension along any axis of the matrix is divisible by the size of its grid along the same axis. For example, $b_1 = n_1 / g_1$ and $b_2 = n_2 / g_2$ are integer values. We call $b_1$ and $b_2$ the dimensions of the blocks of $\X$.

For any matrix multiplication $\C = \A \B$, we have $\A \in \mathbb{R}^{m \times k}$ and $\B \in \mathbb{R}^{k \times n}$ so that $\C \in \mathbb{R}^{m \times n}$. We decompose $\C$ into an $r \times c$ grid. We decompose $\A$ into an $r \times q$ grid and $\B$ into a $q \times r$ grid.
Thus, block $\C_{i,j} = \sum_{h=0}^{q-1} \A_{i,h} \B{h, j}$.

We treat vectors as a special case of the above formulation, with the second axis set to $1$. For example, $\y = \A \x$ is computed by decomposing $\y$ into an $r \times 1$ (column) grid and $\x$ into a $q \times 1$ grid so that $\y_{i} = \sum_{h=0}^{q-1} \A_{i,h} \x_h$.

For element-wise operations, such as $\X + \Y$, we assume that the dimensions of the matrices are equivalent, and the grid into which they're decomposed are also equivalent so that the blocks within the respective grids have compatible dimensions.

\subsubsection{Example: Matrix Multiplication}
\label{sec:matmul-example}

Consider a $6 \times 4$ matrix $\A$ decomposed into blocks of size $2 \times 2$. The grid dimensions of matrix $\A$ are $3 \times 2$.
Let us also define $\B$ as $4 \times 10$ with blocks of size $2 \times 5$ and grid dimensions $2 \times 2$. Note that, in both cases, the element-wise multiplication of the grid and block dimensions yield the dimensions of the entire matrix. To compute the matrix multiplication of $\A$ and $\B$, we proceed as follows.
\begin{align*}
\C & =
\left[\begin{array}{c | c}
    \rule[-2.0ex]{0pt}{5.0ex}
    \sum_{h=0}^{1} \A_{0,h} \B_{h,0} & \sum_{h=0}^{1} \A_{0,h} \B_{h,1}\\
    \hline
    \rule[-2.0ex]{0pt}{5.0ex}
    \sum_{h=0}^{1} \A_{1,h} \B_{h,0} & \sum_{h=0}^{1} \A_{1,h} \B_{h,1} \\
    \hline
    \rule[-2.0ex]{0pt}{5.0ex}
	\sum_{h=0}^{1} \A_{2,h} \B_{h,0} & \sum_{h=0}^{1} \A_{2,h} \B_{h,1}
\end{array}\right] 
 \label{eq:blocks}
\end{align*}
Thus, we represent the $6 \times 10$ matrix $\C$ above as a $3 \times 2$ grid of $ \times 5$ blocks.

\subsection{Distributed Linear Algebra Operations}
\begin{figure}
% \begin{wrapfigure}{r}{0.2\textwidth}
\centering
    \includegraphics[width=0.2\textwidth]{src/figures/block-cyclic.drawio.pdf}
    \caption{Block-cyclic data layout of a matrix $\X$ decomposed into a $3\times4$ grid of blocks, which are distributed over a $2\times2$ grid of nodes. Each color denotes the node on which the block is stored. Nodes $\N_{1,1}, \N_{2,1}, \N_{1,2}, \N_{2,2}$ are the colors blue, green, purple, and yellow, respectively.}
    \label{fig:blk-cyclic}
% \end{wrapfigure}
\end{figure}

Parallelizing block partitioned vectors and matrices can be achieved in a number of different ways. In this section, we describe a simple approach that computes the output blocks of an operation on a grid of {\it nodes}. In this context, nodes may be distinct processes, GPU devices connected on a single computer, or computers that are networked in the cloud.

Let us begin with a grid of $r \times c$ nodes. We have $p = rc$ nodes total. We represent the memory contents of node $i,j$ as the set $\N_{i,j}$.
Each node is unable to access the memory of any other node, and nodes are assumed to have sufficient memory to carry out matrix multiplication on pairs of blocks. How do we decide on which node to store each block that makes up each matrix? How do we decide on which nodes to execute computations?

We decide where each block is stored by assuming a {\it block cyclic data layout}. If $\X$ is decomposed into a $g_1 \times g_2$ grid, then we store $\X_{i,j}$ on node $(i \mod r), (j \mod c)$. 
% Need diagram of block-cyclic.
Note that, when $g_1 = r$ and $g_2 = c$, each block is stored on a distinct node. As for where to execute operations, we will adopt a simple convention: If the output block is in $\N_{i, j}$, then all operations will be performed on node $i, j$.

\subsubsection{Matrix Multiplication}
Recall our general formulation of matrix multiplication of the two matrices $\A$ and $\B$. We have that $\C_{i,j} = \sum_{h=0}^{q-1} \A_{i,h} \B_{h,j}$.
Recall that $b_1 = m / g_1$ and $b_2 = n / g_2$ are the dimensions of each block. We will rewrite the basic procedure for matrix multiplication so that the memory requirements per node are at most $O(b_1 b_2)$. By doing so, we will have a general procedure for matrix multiplication that scales.

In the following algorithms, we write $\forall_{i=0, j=0}^{m-1, n-1} \{ expression \}$ to denote the concurrent execution of $expression$ for all instances of the indices $i \in \{0, \dots, m-1\}$ and $j \in \{0, \dots, n-1\}$.
\begin{algorithm}[h]
\SetAlgoLined
    $\C \gets {\bf 0}$;\\
    \For{$i \gets 0$ \KwTo $m$}{
        \For{$j \gets 0$ \KwTo $n$}{
            \For{$h \gets 0$ \KwTo $k$}{
                $\C_{i,j} \gets \C_{i,j} + \A_{i,h} \B_{h,j}$
            }
        }
    }
\caption{Serial Matrix Multiplication.}
\label{algo:serial}
\end{algorithm}
Consider the approach to matrix multiplication given in Algorithm \ref{algo:serial}. Notice that the operations within the outer two loops (over $i$ and $j$) are all independent of one another. If we reorder the loops and rewrite our matrix multiplication procedure as Algorithm \ref{algo:concurrent}, we can bound the memory required by each node to a constant factor of the block sizes.
\begin{algorithm}
    $\C \gets {\bf 0}$;\\
    \For{$h \gets 0$ \KwTo $k$}{
        $\forall_{i=0, j=0}^{m-1, n-1} \, \{ \C_{i,j} \gets \C_{i,j} + \A_{i,h} \B_{h,j} \}$
    }
\caption{Concurrent Matrix Multiplication.}
\label{algo:concurrent}
\end{algorithm}
Lets assume we have an $m \times n$ grid of nodes on which to execute the above computation. We can see that, for each iteration of the outer loop, we need 1 block to store the result, and 2 blocks to perform the matrix multiplication. Thus, Algorithm \ref{algo:concurrent} provides a way to arbitrarily scale matrix operations.

While we've shown that this approach achieves good scaling, we have not discussed the matter of transmitting blocks between nodes in order to perform the required operations. Recall our simple assumption: If the output block $\C_{i, j}$ is in $\N_{s, t}$, then all operations are performed on $\N_{s, t}$. We'll simply assume that any operation performed on $\N_{s, t}$ transmits the required blocks implicitly from the nodes on which they reside under the block cyclic data layout. It's worth noting that sophisticated data communication algorithms are typically employed to efficiently interleave communication and computation for distributed memory computations such as the one we've described. In many cases, simply transmitting objects to wherever they are needed is sufficient to achieving good scalable performance.

\subsubsection{Element-wise Unary and Binary Operations}
Element-wise unary operations on a matrix $\X$ decomposed into a grid $g_1 \times g_2$ of blocks distributed over a grid of nodes $r \times c$ can be done by simply applying the operations in place. For example, to perform $e^{\X}$, 
if $\X_{i, j}$ is in $\N_{s, t}$, we simply apply $e^{\X_{i, j}}$ on node $\N_{s, t}$.

Since the unary operation transpose drastically rearranges the way blocks are distributed over a grid of nodes, we treat it differently. If a transpose is performed, we {\it fuse} it with the next operation without actually changing the nodes on which the transposed matrix's blocks reside. The transpose is then performed before the operation with which it is fused. For example, if we must perform $\Y = \X^T \X$, instead of updating the data layout of $\X^T$, we keep all the blocks in place and simply perform $\Y_{i, j} = \sum_{h=0}^{k} (\X^T)_{i, h} \X_{h, j}$ and transmit blocks between nodes as needed for the matrix multiply.

For element-wise binary operations between two matrices $\A$ and $\B$, we assume $\A$ has the same dimension and decomposition as $\B$. By the block-cyclic data layout, if $\A_{i,j}$ is in $\N_{s, t}$, so is $\B_{i, j}$, and the operation is performed on node $\N_{s, t}$ without requiring any communication between nodes. Thus, we also have that each output block $\C_{i, j}$ also resides on $\N_{s, t}$. For example, the expression $\C = \A + \B$ induces the computation $\C_{i, j} = \A_{i, j} + \B_{i, j}$ on $\N_{s, t}$.
