# Supplementary material for: NumS: Scalable Array Programming for the Cloud
Source: arXiv:2206.14276 source file (2022-07-13)
Supplement: Supplementary file 2 [file 005-syntax-semantics.tex]

\section{Syntax and Semantics}
\label{appendix:syntax-semantics}

Our API design and implementation are heavily influenced by the formulation we present in this section.
We present the foundations of our API as a formal language, with inductively defined syntax.

We use the syntax of a basic subset of the Python programming language, along with a basic set of systems operations \alvin{what are `systems' operations}, to define a translation operator that translates Python code to a language of concurrently executing futures. We then extend both the source and destination languages, as well as the translation operator, to support 2-dimensional arrays.
While our presentation---our languages, translations, and proofs---are defined for a shared-memory system of concurrently executing futures using the example of 2-dimensional arrays, our implementation is $n$-dimensional and runs on the distributed system Ray \cite{ray}.

We summarize the syntax of our languages, informally describe our semantics, and provide a proof sketch of correctness. 
\alvin{what's the point of this section? are you describing how block / graph arrays are compiled into actual ray code? if so i don't see any mention of that in this section? or how parallelism is extracted from silver code?}

\subsection{Notation}
Much of this section requires a basic understanding of BNF notation, a notation for defining programming languages recursively. While we use the term "programming language" to refer to our source and target languages, much of what we define in this section are key operations required to formulate our translation procedure. The syntax $a ::= constant \mid a_1 \bop a_2$ can be broken down as follows. The variable to the left of $::=$ is a recursive definition of a piece of syntax, while the right side may contain subscripted instances of the variable being defined, as well as other variables that have been previously defined. $\mid$ can be interpreted as "or." In this example, $a$ can be $constant$, or the binary operation $a_1 \bop a_2$. In turn, $a_1$ and $a_2$ can be any piece of syntax that appears in the definition of $a$. We use $\dots$ to denote the operations which appear previously for a particular variable which has already been defined. 

Similar to our language definition, the translation solution we present in this work is defined recursively, where $\equiv$ is used to recursively define the translation of every operator in our source language.
This approach to defining our translation procedure allows us to reason about the runtime behavior and correctness of different translation solutions. \alvin{pls check with others but I don't think this type of explanation is needed based on my DB and PL paper writing experience. The reader is assumed to know what BNF grammars are.}

\subsection{Futures with Concurrency}

\begin{figure}[h]
\begin{align*}
\c \enspace \Coloneqq & \enspace \skipp \sbar \c_1 ; \c_2 \sbar \x = \e \\
& \sbar \iif{\b}{\c_1}{\c_2} \\
& \sbar \while{\b}{\c} \\
\f \enspace \Coloneqq & \enspace \f(\x_1, ..., \x_m)\{\e\}
\end{align*}
\caption{Definition of Sub-Python statements in BNF form. Assignment stores the result
of Python expressions $\e$ as the variable $\x$. $\b$ is defined inductively over Boolean expressions.}
\label{fig:python:syntax}
\end{figure}

\begin{figure}[h]
\begin{align*}
\r \enspace \Coloneqq & \enspace \R(\f) \\
\o \enspace \Coloneqq & \enspace \id{\v_1, ..., \v_m} \sbar \r(\o_1, ..., \o_m) \sbar \putt(\e) \\
\e \enspace \Coloneqq & \enspace \dots \sbar \o \sbar \get(\o)
\end{align*}
\caption{Sub-Python extended to support futures.
The $\R$ operator is a higher-order function that takes as input Python functions
and outputs remote functions.
$\o$ denotes the space of futures, which is comprised
of the $\id{\cdot}$ operator, the output of remote function calls, and the $\putt$ operator.
The space of expressions $\e$ is extended to include futures and the $\get$ operator.
For any value $\v$, we have $\v = \get(\putt(\v))$.}
\label{fig:futures:syntax}
\end{figure}

Our approach to concurrency relies on futures and promises.
A promise can be thought of as a function which executes asynchronously, immediately returning a future. The returned future can be thought of as a reference to the object that the promise computes. When we allow promises to operate on futures, a single-threaded process can execute 
a program comprised of futures and promises without doing any of the computation. The underlying execution model can be anything. In this work, we execute futures concurrently.
To understand this, it's helpful to consider a future as having two states: It's either computed and references an object, or it's not computed and references a promise. \alvin{are promises not objects?} If a promise $\f(x)$ is called with a future $\x$ that has been computed, \alvin{weird. what is the promise here? f? f(x)? x?} the promise is considered {\it independent} \alvin{you mean realized?}. An independent promise can be executed immediately. A promise called with a future $\y$ that has not yet been computed is considered {\it dependent}. In the concurrently executing futures model, all independent promises are executed concurrently. The goal of a concurrently executing futures-based system is to translate a program comprised of futures and promises to concurrently executing code. Our goal in this section is to translate a subset of serial Python code to futures and promises.

The subset of Python we consider is given in figure \ref{fig:python:syntax}.
We call this language {\bf Sub-Python}. Some key operations include loops, conditionals, and functions. Our language of futures, called {\bf Sub-Futures}, is the extension of Sub-Python given in figure \ref{fig:futures:syntax}. Sub-Futures enables concurrent execution of arbitrary functions on shared memory. \alvin{why are there (yet another) two languages here?} This design is heavily inspired by the distributed system Ray \cite{ray}. The operator $\R$ is used to create an RPC from an existing function $\f$. \alvin{you mean call an RPC? what does create mean}
The piece of syntax $\o$ (short for object reference), is used to define the futures of our language: $\id$ constructs the future associated with a collection of values $\v_i$, $r(\o_1, \dots, \o_m)$ denotes the future returned by a call to the RPC $\r$, and $\putt(\e)$ denotes the future returned by submitting the result of an expression to the distributed system store. The set of expressions $\e$ is extended to include futures, and the $\get(\o)$ operation, which retrieves the object associated with the future $\o$. \alvin{sorry I am quite confused. the language shown in fig 1 doesn't look similar to that shown in the code fragments in sec 2}

\subsection{Program Translation}
\label{sec:translation}
Our translation procedure translates all operations from the Sub-Python language to the Sub-Futures language. The key benefit of our translation-based approach is composability: Any composition of operations from Sub-Python can be translated to a semantically equivalent Sub-Futures program. We describe the translation procedure inductively by way of a translation operator $\T$ below.

\vspace{-1.5em}
\begin{align*}
% Commands
\T(\skipp) & \equiv \skipp \\
\T(\c_1 ; \c_2) & \equiv (\T(\c_1); \T(\c_2)) \\
\T(\x = \e) & \equiv \x = \T(\e) \\
% Functions
\T(\f(\x_1, \dots, \x_m)\{\e\}) & \equiv \R(\f(\x_1, \dots, \x_m)\{\e\}) \\
\T(\R(\f)) & \equiv \R(\f) \\
\T(\f(\e_1, \dots, \e_m)) & \equiv \T(\f)(\T(\e_1), \dots, \T(\e_m)) \\
% Binary Operations
\T(\a_1 \bop_2 \a_2) & \equiv \R(\bop_2)(\T(\a_1), \T(\a_2)) \\
\T(\v) & \equiv \putt(\v) \\
\T(\x) & \equiv \x
\end{align*}
\vspace{-1.5em}

Here $\bop_2$ is shorthand for arbitrary binary operations on arithmetic expressions.
This translation operator takes syntax from a subset of Python code and translates it to futures syntax which, when executed by the driver process $\M$,
generates correct programs in our computation model.

\subsection{Correctness}
\label{sec:correctness}
In this section, we provide a proof sketch which shows that Sub-Futures is semantically equivalent to Sub-Python.
Consider key/value stores $\sigma$, $\sigma'$, and $\mu$. \alvin{fig 1 and 2 don't show any key value stores??} In our source language, $\sigma$ maps keys directly to values. In our target language,
$\sigma'$ maps keys to futures, and $\mu$ maps futures to values.
The basic idea behind our proof is as follows: If some program from the source language terminates with store content $\sigma$, then the target language must also terminate with store contents $\sigma'$ and $\mu$ such that for any key/value pair $(\x, \v) \in \sigma$, there exists 
$(\x, \o) \in \sigma'$ and $(\o, \v) \in \mu$.
For instance, if we evaluate the assignment operation $\x = 1 + 2$ in our source language, we end up with some value $(\x, 3) \in \sigma$.
According to our translation operator, we want our source language translated as $\x = \R(+)(\o_1, \o_2)$. The semantics of our RPC calls dictate that the expression $\R(+)(\o_1, \o_2)$ evaluates to $\o_3$ such that $(\o_3, \v) \in \mu$, and the assignment yields $(\x, \o_3) \in \mu$.

\subsection{2-Dimensional Futures}

Consider a snippet of our NumPy-inspired array syntax.
We focus on the matrix multiplication operator,
which is the only binary operation which does not
trivially generalize to $n$ dimensions.
\begin{align*}
\A \enspace \Coloneqq & \enspace \N(n, m) \sbar \x \sbar \dots \sbar \A_1 @ \A_2
\end{align*}

We have $\A \in \mathcal{A}$, where $\mathcal{A}$ is the set 
defined above in BNF form, and $\N(n, m) \in \mathbb{R}^{n \times m}$ is a
real-valued 2-dimensional array.
To translate arrays to our target language,
we will need a way to represent them as futures.
We define the syntax for a 2-dimensional array of futures as follows.
\begin{align*}
\o \enspace \Coloneqq & \enspace \dots \sbar \o(\kappa_1, \kappa_2)
\end{align*}
The syntax $\o(\kappa_1, \kappa_2)$ denotes a 2-dimensional futures encoding
of 2-dimensional arrays, where $\kappa_1, \kappa_2$ define the number of
blocks along axes $1$ and $2$.
To ease the exposition of our treatment of arrays, assume that $\kappa_1 = n$
and $\kappa_1 = m$,
so that every value $\v_{i,j}$ in $\N(n, m)$ is translated to a future $\o_{i, j}$
in $\o(n, m)$.
The structure of 2-dimensional futures is as follows:
\begin{align}
\o(n, m) & =
\begin{bmatrix}
    \o_{1, 1} & \dots & \o_{1, m}  \\
    \vdots & \ddots & \vdots \\
     \o_{n, 1} & \dots & \o_{n, m}.
 \end{bmatrix}
\end{align}
We call 2-dimensional arrays of futures {\it 2-dimensional futures} for short.
For our translation of matrix multiplication,
we denote by $\x_1, \N_1(n_1, m_1), \o_1(n_1, m_1)$
the operands corresponding to the left-hand side of the $\mm$ operation,
and by $\x_2, \N_2(n_2, m_2), \o_2(n_2, m_2)$ the right-hand side.
The result is denoted by $\N(n, m)$ and $\o(n, m)$, where $n=n_1$ and $m=m_2$.
We use the notation $\o_1(n_1, m_1)_{i, :}$ and $\o_1(n_1, m_1)_{:, j}$
to denote the $i$th row and $j$th column of $\o_1$, respectively.
The local function $\g(\args_{i,j})$ computes the $i,j$ entry of
the result $\N(n, m)$, 
where $\args_{i,j} = (\o_1(n_1, m_1)_{i, :}, \o_2(n_2, m_2)_{:, j}, i, j)$.
We define $\g$ as follows:
\begin{align*}
    \g(\args_{i,j}) \equiv  & \R(+)( \\
    & \R(\mm)(\o_1(n_1, m_1)_{i, 1}, \o_2(n_2, m_2)_{1, j}) \,, \\
    & \dots \,, \, \\
    & \R(\mm)(\o_1(n_1, m_1)_{i, k}, \o_2(n_2, m_2)_{k, j})),
\end{align*}
where $k = m_1 = n_2$.
The translation operator for matrix multiplication is as follows:
\begin{gather*}
\T(\o_1(n_1, m_1) \mm \o_2(n_2, m_2))  \equiv \\
\qquad \qquad \begin{bmatrix}
    \g(\args_{1,1}) & \dots & \g(\args_{1, m}) \\
    \vdots & \ddots & \vdots \\
    \g(\args_{n, 1}) & \dots & \g(\args_{n, m})
\end{bmatrix} \\
\T(\x_1 \mm \x_2)  \equiv \T(\T(\x_1) \mm \T(\x_2)).
\end{gather*}
Each entry $\o_{i, j}$ in array $N(n, m)$
is computed using remote functions. While this 
is inefficient due to the RPC overhead problem,
it illustrates our approach to parallelizing array operations.

The correctness of matrix multiplication follows from our proof of
correctness of functions. Each entry of the matrix
is computed by a composition of basic linear algebra operations on
futures. Our translation operator generates $n \times m$
such remote function compositions to generate each future entry of $\o(n, m)$.
The resulting 2-dimensional futures object therefore contains entries
such that for each value $\v_{i,j}$ in $\N(n, m)$ computed by a Python program, we have $(\o_{i,j}, \v_{i,j}) \in \mu$.

\subsection{Data Dependency Resolution and Concurrency}
\alvin{what's the connection with the previous section?}
The 2-dimensional futures object solves the data dependency problem of matrix multiplication by translating all values to futures, and all binary operations 
to RPCs. The semantics of our execution model is defined on $k$ worker processes. Futures generated by RPCs are computed on workers, which block until the futures on which they depend are made available. Let $k$ go to infinity. In this configuration, all operations which have no dependencies execute concurrently, and all operations which have dependencies block until their dependencies are resolved. Thus, our formulation of 2-dimensional futures simultaneously solves the data dependency and concurrency problem.

\subsection{N dimensions and Distributed Memory}
\label{sec:ext-distr-mem}
% Much of the text below may be redundant.
\paragraph{N-Dimensions}
The correctness of all but matrix multiplication trivially extends 
to the $n$-dimensional setting.
We now describe how our translation approach and proof of
correctness generalizes to the $\tensordot(\A_1, \A_2, n)$ operation. Consider the output shape of a matrix multiply of two arrays $\N_1(n_1, m_1)$ and $\N_2(n_2, m_2)$. The output shape $(n_1, m_2)$ provides a structure whereby the correct value of each entry $\N(n_1, m_2)_{i,j}$ is a basic sum of products. The same idea applies to the \tensordot\  operation: The output structure (shape) of a tensor dot operation is predefined.
% The computation of each entry of the output of a tensor dot can be thought of as an independent composition of basic arithmetic operations.
Consider the output of the \tensordot\  operation, an n-dimensional array $\N$.
Let $\I$ denote the index tuple which accesses arbitrary entries
of an n-dimensional array, so that $\v_{\I} \in \mathbb{R}$ is a value in $\N$.
The \tensordot\ operation is a straightforward
generalization of matrix multiplication. 
Like matrix multiplication, each entry $\v_{\I}$ is computed
by a composition of binary functions.
Thus, each entry $\o_{\I}$ in an n-dimensional futures object is a composition of remote functions. The proof argument is the same as the proof for 2-dimensional arrays.

% TODO: Improve this.
\paragraph{Distributed Memory}
While we do not model distributed memory explicitly, we informally show that our approach can be extended to the distributed-memory setting. \alvin{why bother? is this something that you have implemented?}

Consider the key/value stores introduced in Section \ref{sec:correctness}:
$\sigma$, $\sigma'$, and $\mu$. We introduce a new key/value store, $\omega$, which maps futures $\o$ to nodes $\eta$, where $\eta$ serves as an identifier corresponding to a set of workers which operate locally on the key/value store $\mu$.
An RPC call with a result associated with future $\o$ is assigned to a worker on node $\eta$. We therefore set $(\o, \eta) \in \omega$. During dependency resolution, a worker will block until $\o$ exists in $\omega$ instead of blocking until $\o$ exists in $\mu$. We make this change because the data may no longer be co-located with the worker executing the RPC. To obtain all future and value pairs $(\o, \v)$ required to execute an RPC, a worker initiates a read from a non-local object store $\mu'$ and writes $\o$ with associated value $\v$ to its local object store $\mu$. The worker then executes the RPC.

Our correctness theorem is extended to include $\omega$ as follows. Consider a cluster with $p$ nodes $\eta_1, \dots, \eta_p$.
We have $p$ stores local to each node, defined as $\mu_1, \dots, \mu_p$.
If some program from the source language terminates with store content $\sigma$, then the target language must also terminate with store contents $\sigma'$, $\mu_i$, and $\omega$ such that for any key/value pair $(\x, \v) \in \sigma$, there exists $(\o, \eta_i) \in \omega$, $(\o, \v) \in \mu_i$, and $(\x, \o) \in \sigma'$.
With minor modifications to the semantics of RPCs as described above, the proof of correctness for the distributed memory setting is very similar to our existing proof.
