# Supplementary material for: NumS: Scalable Array Programming for the Cloud
Source: arXiv:2206.14276 source file (2022-07-13)
Supplement: Supplementary file 3 [file 020-python.tex]

\section{Sub-Python}
\label{appendix:python}

\subsection{Syntax}

In the Python-inspired grammar below, we use curly braces to scope functions,
and semi-colons to delimit statements (commands).

\begin{align*}
\c \enspace \Coloneqq & \enspace \skipp \sbar \c_1 ; \c_2 \sbar \x = \e \sbar \iif{\b}{\c_1}{\c_2} \sbar \while{\b}{\c} \\
\e \enspace \Coloneqq & \enspace \a \sbar \b \sbar \f \sbar \f(\e_1, ..., \e_m) \sbar \mathbf{null} \\
\f \enspace \Coloneqq & \enspace \f(\x_1, ..., \x_m)\{\e\} \\
\a \enspace \Coloneqq & \enspace \n \sbar \x \sbar -\a \sbar \a_1 + \a_2 \sbar \a_1 - \a_2 \sbar \a_1 * \a_2 \sbar \a_1 + \a_2 \\
\b \enspace \Coloneqq & \enspace \true \sbar \false \sbar \x \sbar \mathbf{not} \ \b \sbar \b_1 \ \mathbf{or} \ \b_2 \sbar \b_1 \ \mathbf{and} \ \b_2 \sbar \a_1 == \a_2 \sbar \a_1 < \a_2 \\
\v \enspace \Coloneqq & \enspace \true \sbar \false \sbar \n \sbar \f \\
\d \enspace \Coloneqq & \enspace \v \sbar \mathbf{error}
\end{align*}
\iffalse
\begin{verbatim}
c ::= skip | c_1 ; c_2 | x = e | if b then c_1 else c_2 | while b do c 
e ::= a | b | f | f(e_1, ..., e_m) | null
f ::= f(x_1, ..., x_m){e} 
a ::= n | x | -a | a_1 + a_2 | a_1 - a_2 | a_1 * a_2 | a_1 + a_2 
b ::= True | False | x | not b | b_1 or b_2 | b_1 and b_2 | a_1 == a_2 | a_1 < a_2 
v ::= True | False | n | f
d ::= v | error
\end{verbatim}
\fi
Evaluation order is defined as follows.
\begin{align*}
\ARG \enspace \Coloneqq & \enspace \e \sbar \e \ , \ \ARG \\
\H \enspace \Coloneqq & \enspace \mathbf{[.]} \sbar \mathbf{not} \ \H \sbar -\H \sbar \H \bop \e \sbar \v \bop \H \sbar \f(\H) \sbar \H\ ,\ \ARG \sbar \v \ ,\ \H
\end{align*}
% what is \bop
\iffalse
\begin{verbatim}
ARG ::= e | e, ARG
H   ::= [.] | not H | -H | H \bop e | v \bop H | f(H) | H, ARG | v, H
\end{verbatim}
\fi
Above, $\bop$ ranges over Boolean and arithmetic binary operations.
We introduce $\d$ above to deal with cases where expressions evaluate to either a value $\v$ or $\nulll$.

\subsection{Semantics} 
The semantics for this grammar are equivalent to small-step operational semantics of IMP \cite{winskel}. 
The program state $\sigma$ is not type-safe.
We allow for $\bot \in \Sigma$ to indicate non-terminating programs.
In what follows, 
we define the semantics for terminating and non-terminating expressions (due to recursion), as well as functions.
Let $\rightarrow^k$ denote $k$ small steps, and $\mathcal{V}$ denote the set of values. We define $\d \in \mathcal{V} \cup \{ \nulll \}$.

\begin{mathpar}
  \inferrule*[Right=Expr]{
  \exists k. \, H[\e] \rightarrow^k H[\v]
  }{
    \br{H[\e], \sigma} \rightarrow^{*} \br{H[\v], \sigma}
  }

  \inferrule*[Right=Expr-$\infty$]{
  \forall k. H[\e] \rightarrow^k H[\e'] \and \e' \notin \mathcal{V}
  }{
    \br{H[\e], \sigma} \rightarrow \br{\nulll, \sigma}
  }
\end{mathpar}

\begin{mathpar}
  \inferrule*[Right=Assgn-$\infty$]{
    \e \rightarrow \nulll
  }{
    \br{\x = \e, \sigma} \rightarrow \br{\skipp, \bot}
  }
  \\
  \inferrule*[Left=Assgn]{
    \e \rightarrow^{*} \v
  }{
    \br{\x = \e, \sigma} \rightarrow \br{\skipp, \sigma[\x = \v]}
  }
  \inferrule*[Right=Assgn-Dead]{
    \e \rightarrow^{*} \d
  }{
    \br{\x = \e, \bot} \rightarrow \br{\skipp, \bot}
  }
  \\
  \inferrule*[Left=Read]{
    \sigma(\x) = \v
  }{
    \br{\x, \sigma} \rightarrow \br{\v, \sigma}
  }
  \inferrule*[Right=Read-Dead]{
  }{
    \br{\x, \bot} \rightarrow \br{\nulll, \bot}
  }
  \\
  \inferrule*[Right=Cmd-$\infty$]{
  }{
    \br{\c, \bot} \rightarrow \br{\skipp, \bot}
  }
\end{mathpar}

\begin{mathpar}
  \inferrule*[Right=Func-Eval]{
    \br{\e_i, \sigma} \rightarrow^{*} \br{\v_i, \sigma} \and
    \br{[\v_i/\x_i]_{i=1}^{m} \, \e, \sigma} \rightarrow^{*} \br{\v, \sigma}
  }{
    \br{\f(\x_1, \dots, \x_m)\{\e\}(\e_1, \dots, \e_m), \sigma} \rightarrow^{*} \br{\v, \sigma}
  }
\end{mathpar}

Note that in the rule for non-terminating expressions, the entire context transitions to $\nulll$,
which covers cases such as $\nulll + \e$, $\f(\nulll, \dots, \e_m)$, etc.
We have reads on $\bot$ evaluate to $\nulll$ to be consistent with read behavior in the multi-process setting.

\subsubsection{Loop Semantics}
We define the semantics of while loops in terms of a bounded while loop which executes
at most $k$ times before transitioning to $\bot$, written $\whilek{k}{\b}{\c}$. The
operational semantics of ${\bf while_k}$ is defined as follows.

\begin{mathpar}
  \inferrule*[Right=While-0]{
    \br{\b, \sigma} \rightarrow \br{\true, \sigma}
  }{
    \br{\whilek{0}{\b}{\c}, \sigma} \rightarrow \br{\skipp, \bot}
  }
  \\
  \inferrule*[Right=While-k-True]{
      \br{\b, \sigma} \rightarrow \br{\true, \sigma} \and
      k > 0
  }{
    \br{\whilek{k}{\b}{\c}, \sigma} \rightarrow \br{\c ; \whilek{k-1}{\b}{\c}, \sigma}
  }
  \\
  \inferrule*[Right=While-k-False]{
      \br{\b, \sigma} \rightarrow \br{\false, \sigma}
  }{
    \br{\whilek{k}{\b}{\c}, \sigma} \rightarrow \br{\skipp, \sigma}
  }
\end{mathpar}

The semantics for ${\bf while_k}$ can be interpreted simply as follows: 
If after $k$ executions of $\c$ the conditional $\b$ still evaluates to $\true$,
then transition the program state to $\bot$. We use this key
property of ${\bf while_k}$ below to define the semantics of ${\bf while}$ 
to handle non-terminating programs.

\begin{mathpar}
  \inferrule*[Right=While-True]{
      \br{\b, \sigma} \rightarrow \br{\true, \sigma} \and
      \exists k . \,
      \br{\whilek{k}{\b}{\c}, \sigma} \rightarrow^{*} \br{\skipp, \sigma'} \and 
      \sigma' \neq \bot
  }{
    \br{\while{\b}{\c}, \sigma} \rightarrow \br{\c ; \while{\b}{\c}, \sigma}
  }
  \\
  \inferrule*[Right=While-$\infty$]{
      \forall k . \,
      \br{\whilek{k}{\b}{\c}, \sigma} \rightarrow^{*} \br{\skipp, \bot}
  }{
    \br{\while{\b}{\c}, \sigma} \rightarrow \br{\skipp, \bot}
  }
  \\
  \inferrule*[Right=While-False]{
      \br{\whilek{k}{\b}{\c}, \sigma} \rightarrow \br{\skipp, \sigma}
  }{
    \br{\while{\b}{\c}, \sigma} \rightarrow \br{\skipp, \sigma}
  }
\end{mathpar}

The derivation \textbf{While-True} can be interpreted as follows: When $\b$ evaluates to $\true$, if there is some $k$ for which $\whilek{k}{\b}{\c}$ transitions to a program state other than $\bot$, then $\while{\b}{\c}$ is terminating and can make progress.
The derivation \textbf{While-$\infty$} simply states that if no $k$ exists such that
$\whilek{k}{\b}{\c}$ terminates in a state other than $\bot$, 
then the loop $\while{\b}{\c}$ cannot make progress and yields state $\bot$.
The derivation of \textbf{While-False} is self-evident.

% \begin{mathpar}
%   \inferrule*[Right=For-in-n]{
%     \n_1 < \n_2 - 1
%   }{
%     \br{\forr{\ii}{\n_1}{\n_2}{\c}, \sigma} \rightarrow \br{(\ii=\n_1 ; \c ; \dots ; \ii=\n_2-1 ; \c), \sigma}
%   }
%   \\
%   \inferrule*[Right=For-in-1]{
%     \n_1 = \n_2 - 1
%   }{
%     \br{\forr{\ii}{\n_1}{\n_2}{\c}, \sigma} \rightarrow \br{(\ii=\n_1 ; \c, \sigma}
%   }
%   \\
%   \inferrule*[Right=For-in-0]{
%     \n_1 >= \n_2
%   }{
%     \br{\forr{\ii}{\n_1}{\n_2}{\c}, \sigma} \rightarrow \br{\skipp, \sigma}
%   }
% \end{mathpar}
