# Supplementary material for: NumS: Scalable Array Programming for the Cloud
Source: arXiv:2206.14276 source file (2022-07-13)
Supplement: Supplementary file 4 [file 030-futures.tex]

\section{Futures}
\label{appendix:futures}

We define a futures-based extension of the Sub-Python language,
called Sub-Futures, 
which provides an API enabling concurrent execution of arbitrary functions on a shared memory store.
We adopt much of the syntax from
Dijkstra's language of guarded commands,
Hoare and Milner's language of communicating processes,
and Milner's CCS. 

We define the configuration of a futures program with $k$ workers
as follows:
\begin{align}
  \rayop{\M}{\W}{\S}{\sigma, \mu},
\end{align}
where $\M$ denotes the main futures process (aka the driver),
$\sigma$ denotes the state for $\M$,
$\S = \S^r \dbar \S^{w} = \S^r_0 \dbar \S^r_1 \dbar ... \dbar \S^r_k \dbar \S^{w}$
denotes a collection of "store" processes which are responsible for
writing to and reading from a shared state $\mu$ across all processes,
called the store, and $\W = \W_1 \dbar ... \dbar \W_k$ denotes $k$ worker processes.

\subsection{Futures: Communication Syntax}

This section and the next can be skipped if the reader is already familiar with these languages.
Duplication of some of the operations is necessary to ensure correct 
semantics when defining transitions between command operations
and operations which evaluate to data.
$\s$ is used to label an arbitrary channel of communication, and
$\tau$ is the null process and is equivalent in functionality to $\skipp$ for commands.
\\\\
\textbf{Communication Commands:}
\begin{align*}
\c \enspace \Coloneqq & \enspace ... \\
& \sbar \s!\mu(\o) \\
& \sbar \seal(\o, \f(\e_1, ..., \e_m)) \\
& \sbar \sealed(\o) \ =>\  \c \\
& \sbar \gc \\
& \sbar \mathbf{do} \ \gc \ \mathbf{od}
\end{align*}
\textbf{Guarded commands:}
\begin{align*}
\gc \enspace \Coloneqq & \enspace \s?(\x_1, ..., \x_m) \ => \ \c \\
& \sbar \sum(\s_0?(\x_1, ..., \x_m) \ => \ \c_0, ..., \s_k?(\x_1, ..., \x_m) \ => \ \c_k) \ => \ \c_k 
\end{align*}
\textbf{Communication Operations:}
\begin{align*}
\p \enspace \Coloneqq & \enspace \tau \sbar \wait(\o) \sbar \snd(\o) \sbar \rcv(\o) \sbar \seal(\o, \v) \\
& \sbar \s!(\v_1, ..., \v_m) \sbar \s?(\x_1, ..., \x_m) \ => \ \p \\
& \sbar \p \ => \ \p \sbar \p \ => \ \v
\end{align*}

\iffalse
\begin{verbatim}
# Communication Commands.
c ::= ...
    | s!\mu(o)
    | seal(o, f(e_1, ..., e_m))
    | sealed(o) => c
    | gc
    | do gc od

# Guarded commands.
gc ::= s?(x_1, ..., x_m) => c
     | sum(s_0?(x_1, ..., x_m) => c_0, ..., s_k?(x_1, ..., x_m) => c_k) => c_k

# Communication Operations.
p ::= \tau | wait(o) | snd(o) | rcv(o) | seal(o, v)
    | s!(v_1, ..., v_m) | s?(x_1, ..., x_m) => p
    | p => p | p => v
\end{verbatim}
\fi

% \begin{bnfgrammar}
% \c ::= $\dots$
%     | $\s \, ! \, \mu(\o)$
%     | $\seal(\o, \f(\e_1, ..., \e_m))$
%     | $ \sealed(\o) => \c $
%     | $\gc$
%     | $\dood{\gc}$
% \end{bnfgrammar}

% \begin{bnfgrammar}
% $\gc$ ::= $\s \, ? \, (\x_1, ..., \x_m) => \c$
%     | $\sum_{i=0}^{k} \s_i \, ? \, (\x_1, ..., \x_m) \Rightarrow \c_i$
% \end{bnfgrammar}

% \begin{bnfgrammar}
% $\p$ ::= $\tau$ | $\wait(\o)$ | $\snd(\o)$ | $\rcv(\o)$ | $\seal(\o, \v)$
%     | $\s \, ! \, (\v_1, ..., \v_m)$ | $\s \, ? \, (\x_1, ..., \x_m) => \p$
%     | $\p => \p$ | $\p => \v$
% \end{bnfgrammar}

Following are some clarifications on transitions.
\begin{enumerate}
    \item Worker and store processes rely on the \verb|do gc od| command in
    order to invoke commands on incoming data.
    This is also why we've defined the special commands 
    $\seal(\cdot)$, $\sealed(\cdot)$ and $\s!\mu(\cdot)$, 
    as these are downstream commands to the guarded commands.
    \item The semantics for $\get(\cdot)$, $\putt(\cdot)$, and $\R(f)(\cdot)$
    transition through a sequence of communication operations, all of which
    have defined semantics, and all of which eventually transition to either
    a value or an object id.
    \item $\wait, \snd, \rcv,$ and $\seal$ are aliases
    to communication operations to improve the readability of 
    semantics, proofs, etc.
\end{enumerate}

\subsection{Futures: Communication Semantics}

Assume the following.
\begin{enumerate}
  \item Whenever a command transitions to "nothing," it transitions to $\skipp$.
  \item Whenever a process transitions to "nothing," it transitions to $\tau$.
\end{enumerate}

\begin{mathpar}
  \inferrule*[Right=Send]{
  }{
    \xstep{\s \, ! \, (\v_1, ..., \v_m)}{\s \, ! \, (\v_1, ..., \v_m)}{\p}
  }
  \\
  \inferrule*[Right=Rcv]{ }{
    \xstep{\s \, ? \, (\x_1, ..., \x_m) \Rightarrow \p}{\s \, ? \, (\v_1, ..., \v_m)}{\p[\v_1/\x_1, ..., \v_m/\x_m]}
  }
  \\
  \inferrule*[Right=Send-Value-Cmd]{
    \mu(\o) = \v
  }{
    \comstep{\s \, ! \, \mu(\o)}{\sigma, \mu}{\s \, ! \, \v}{\c}{\sigma', \mu'}
  }
  \\
  \inferrule*[Right=Rcv-Guard-Cmd]{ }{
    \comstep{\s \, ? \, (\x_1, ..., \x_m) \Rightarrow \c}{\sigma, \mu}{\s \, ? \, (\v_1, ..., \v_m)}{\c[\v_1/\x_1, ..., \v_m/\x_m]}{\sigma', \mu'}
  }
  \\
  \inferrule*[Right=Rcv-Sum-Guard-Cmd]{
    \comstep{\s_j \Rightarrow \c_j}{\sigma, \mu}{\s_j?(\v_1, ..., \v_m)}{\c_j}{\sigma', \mu'}
  }{
    \comstep{\sum_{i=0}^{k} \s_i ? (\x_1, ..., \x_m) \Rightarrow \c_i}{\sigma, \mu}{\lambda}{\c_j}{\sigma', \mu'}
  }
  \\
  \inferrule*[Right=Loop-Guard-Cmd]{
    \comstep{\gc}{\sigma, \mu}{\lambda}{\c}{\sigma, \mu}
  }{
    \comstep{\dood{\gc}}{\sigma, \mu}{\lambda}{\c ; \dood{\gc}}{\sigma', \mu'}
  }
\end{mathpar}

\subsection{Sub-Futures Syntax}

In the following, we'll define the syntax of Sub-Python extended with the futures API,
and additional syntax to support inter-process communication and parallelism.
Sub-Futures schedules remote functions by selecting worker processes at random, and maintaining a single centralized object store.
Much of the design of Sub-Futures is inspired by distributed systems such as Ray and Dask \cite{ray, dask}.

The syntax for declaring a remote function $\r$
using an existing function $\f$ is defined by the syntax $\R(\f)$.
When a remote function is invoked with $r(\o_1, \dots, \o_m)$,
the function evaluates on a separate process and execution 
on the process which invoked the remote function continues
to make progress. $\putt(\e)$ puts data in the object store
and returns an object id $\o$, and $\get(\o)$ 
gets an object from the object store and returns a value $\v$.
The $\id{\cdot}$ function is not part of the Sub-Futures API, but is needed
internally to generate hashes of objects and function invocations.
The Sub-Futures API and $\id{\cdot}$ function are defined as follows.
\\\
\textbf{Sub-Futures Extensions:}
\begin{align*}
\o \enspace \Coloneqq & \enspace \id{\v_1, ..., \v_m} \sbar \r(\o_1, ..., \o_m) \sbar \putt(\e) \\
\c \enspace \Coloneqq & \enspace ... \sbar \o \ = \ \v \\ 
\r \enspace \Coloneqq & \enspace \R(\f) \\
\a \enspace \Coloneqq & \enspace ... \sbar \rand(\a) \\
\e \enspace \Coloneqq & \enspace ... \sbar \o \sbar \get(\o) \\
\v \enspace \Coloneqq & \enspace ... \sbar \id{\v_1, ..., \v_m} \\
\h \enspace \Coloneqq & \enspace ... \sbar \putt(\H) \sbar \get(\H) \sbar \r(\H) \\
\end{align*}
\textbf{Parallelism:}
\begin{align*}
\h \enspace \Coloneqq & \enspace \c \sbar \c \ ||\  \h
\end{align*}

\iffalse
\begin{verbatim}
# Sub-Futures Extensions.
o ::= id(v_1, ..., v_m) | r(o_1, ..., o_m) | put(e) 
c ::= ... | o = v 
r ::= R(f) 
a ::= ... | rand(a) 
e ::= ... | o | get(o) 
v ::= ... | id(v_1, ..., v_m)
H ::= ... | put(H) | get(H) | r(H)

# Parallelism.
h ::= c | c || h
\end{verbatim}
\fi

The syntax $\o = \v$ adds values to $\mu$
so that $(\o, \v) \in \mu$ and $\mu(\o)$ evaluates to $\v$.

%%%%%%%%%%%%%%%%%
% SEMANTICS
%%%%%%%%%%%%%%%%%

\subsection{Sub-Futures Semantics}

In this section we present semantics for the Sub-Futures API and parallelism.
We continue with small-step operational semantics.
The state $\sigma$ is initialized to $\{k = \n\}$,
where $\n$ corresponds to the number of Sub-Futures workers.
\begin{mathpar}
  \inferrule*[Right=Store-Assgn-$\infty$]{ }{
    \raystep{\o=\nulll}{\sigma, \mu}{\skipp}{\sigma, \bot}
  }
  \\
  \inferrule*[Left=Store-Assgn]{ }{
    \raystep{\o=\v}{\sigma, \mu}{\skipp}{\sigma, \mu[\o=\v]}
  }
  \inferrule*[Right=Store-Assgn-Error]{ }{
    \raystep{\o=\v}{\sigma, \bot}{\skipp}{\sigma, \bot}
  }
  \\
  \inferrule*[Left=Store-Read]{
    \mu(o) = \v
  }{
    \raystep{\mu(o)}{\sigma, \mu}{\v}{\sigma, \mu}
  }
  \inferrule*[Right=Store-Read-Error]{
  }{
    \raystep{\mu(o)}{\sigma, \bot}{\nulll}{\sigma, \bot}
  }
\end{mathpar}

\subsubsection{Assumptions}

The following assumptions are made explicit in the remaining semantics.
Recall that $\M$ is the main process,
$\S = \S^r \dbar \S^{w} = \S^r_0 \dbar \S^r_1 \dbar ... \dbar \S^r_k \dbar \S^{w}$
are store processes,
and $\W = \W_1 \dbar ... \dbar \W_k$ are worker processes.
\begin{enumerate}
  \item $\M$ sends data with $\putt$ to $\S^w$ via communication channel $\alpha_0$.
  \item $\W_i$ sends data with $\seal$ to $\S^w$ via communication channel $\alpha_i$ for $i=1, ..., k$.
  \item $\M$ receives data with $\get$ from $\S^r_0$ via communication channel $\gamma_0$.
  \item $\W_i$ receives data with $\get$ from $\S^r_i$ via communication channel $\gamma_i$ for $i=1, ..., k$.
  \item $\M$ triggers RPCs on $\W_i$ via communication channel $\beta_i$ for $i=1, ..., k$.
  \item Only $\M$ reads from and writes to $\sigma$.
  \item Only $\S$ reads from and writes to $\mu$.
  \item Processes $\W$ and $\S$ have no {\bf local} state.
\end{enumerate}

\subsubsection{Parallelism}

The store processes $\S^r_i$ are responsible for handling reads from the object store.
We parallelize communication from $\M$ and each worker $\W_j$ for $j=1 \dots, k$
to the store processes $\S^r_i$ for $i=0, \dots, k$,
to avoid deadlock,
as well as to prevent the main process and worker processes from
blocking one another.
These semantics are defined as follows:
\begin{mathpar}
  \inferrule*[Right=Parallel-Main]{
    \raystep{\M}{\sigma, \mu}{\M'}{\sigma', \mu}
  }{
    \raystep{\M \dbar \W \dbar \S}{\sigma, \mu}{\M' \dbar \W \dbar \S}{\sigma', \mu}
  }
  \\
  \inferrule*[Right=Parallel-Worker]{
    \raystep{\W}{\sigma, \mu}{\W'}{\sigma, \mu}
  }{
    \raystep{\M \dbar \W \dbar \S}{\sigma, \mu}{\M \dbar \W' \dbar \S}{\sigma, \mu}
  }
  \\
  \inferrule*[Right=Parallel-Store]{
    \raystep{\S}{\sigma, \mu}{\S'}{\sigma, \mu'}
  }{
    \raystep{\M \dbar \W \dbar \S}{\sigma, \mu}{\M \dbar \W \dbar \S'}{\sigma, \mu'}
  }
\end{mathpar}

For non-terminating commands and expressions occurring in $\M$, we have
\begin{mathpar}
  \inferrule*[Right=Parallel-Main-Error]{
  }{
    \raystep{\skipp \dbar \W \dbar \S}{\bot, \mu}{\skipp \dbar \W' \dbar \S'}{\bot, \bot}
  }
  \\
  \inferrule*[Right=Parallel-Main-Error-2]{
  }{
    \raystep{\skipp \dbar \W \dbar \S^r \dbar \o = \d}{\bot, \mu}{\skipp \dbar \W' \dbar \S'}{\bot, \bot}
  }
\end{mathpar}
% In this case, $\W'$ is stateless, but $\S$ may be writing to $\mu$. 
% We define this case explicitly. If $\S = \S^r \dbar \o = \v$, then the parallel program jointly transitions to  $\br{\skipp \dbar \W' \dbar \S', (\bot, \bot)}$. The other case is handled 
% correctly by the semantics of store assignment.

For non-terminating expressions occurring in $\W_i$, we have some function transitioning to $\nulll$. In this case, 
the write process $S^w$ will attempt $\o = \nulll$, which will transition
$\mu$ to $\bot$, and whenever $\mu$ is $\bot$, all assignments $\o = \v$ transition $\bot$ to $\bot$. We therefore define the following parallel semantics to deal with this scenario.
\begin{mathpar}
  \inferrule*[Right=Parallel-Worker-$\infty$]{
  }{
    \raystep{\M \dbar \W \dbar \S^r \dbar \o = \nulll}{\sigma, \mu}{\M \dbar \W' \dbar \S'}{\sigma, \bot}
  }
  \\
  \inferrule*[Right=Parallel-Store-Error]{
  }{
    \raystep{\M \dbar \W \dbar \S}{\sigma, \bot}{\skipp \dbar \W' \dbar \S'}{\bot, \bot}
  }
  \\
  \inferrule*[Right=Parallel-Store-Error-2]{
  }{
    \raystep{\x = \d \dbar \W \dbar \S}{\sigma, \bot}{\skipp \dbar \W' \dbar \S'}{\bot, \bot}
  }
\end{mathpar}
% We have the same problem as above. If $\M$ is assigning to $\sigma$, then we handle
% the parallel transition in the same way as above. Once $\sigma$ transitions to $\bot$,
% $\M$ will transition to $\skipp$.
% We see that whenever such commands / expressions are encountered in the main process or worker process,
% both states transition to $\bot$.

\subsubsection{Worker Processes}

A worker process $\W_i$ is defined as follows. Operational semantics for these processes
appear in the section on remote procedure calls.
\begin{align}
  \W_i = \dood{ \beta_i \, ? \, (\x_f, \x_r, \x_1, \dots, \x_{m}) \Rightarrow \seal(\x_r, \x_f (\get(\x_1), \dots, \get(\x_{m}))) }
\end{align}
This process receives function calls from the main process, executes them, then sends the result
with the appropriate object id to the object store by invoking the $\seal$ operation.

\subsubsection{Store Processes}

Store processes are defined as
$\S = \S^r \dbar \S^{w} = \S^r_0 \dbar \S^r_1 \dbar ... \dbar \S^r_k \dbar \S^{w}$,
where for $i=0, ..., k$ we have
\begin{align}
  \S^r_i &= \dood{ \gamma_i \, ? \, \x \Rightarrow \sealed(\x) \Rightarrow \gamma_i \, ! \, \mu(\x) } \\
  \S^{w} &= \dood{ \sum_{j=0}^{k} \alpha_j \, ? \, (\x_o, \x_v) \Rightarrow \x_o = \x_v  }
\end{align}

The $\sealed$ operation checks whether an object is currently stored in the object store:
\begin{mathpar}
  \inferrule*[Right=Sealed-True]{
    \exists \, \v. (\o, \v) \in \mu
  }{
    \comstep{\sealed(\o) => \c}{\mu}{\lambda}{\c}{\mu'}
  }
  \\
  \inferrule*[Right=Sealed-False]{
    \not\exists \, \v. (\o, \v) \in \mu
  }{
    \comstep{\sealed(\o) => \c}{\mu}{\lambda}{\sealed(\o) => \c}{\mu'}
  }
  \\
  \inferrule*[Right=Sealed-Error]{
  }{
    \comstep{\sealed(\o) => \c}{\bot}{\lambda}{\c}{\bot}
  }
\end{mathpar}
Note that when $\mu=\bot$, all $S^r_i$ processes transmit $\nulll$. Together with semantics for
assignment to $\mu$ and $\sigma$, this behavior causes worker processes to immediately evaluate to $\nulll$, and the main process to enter $\skipp$ with $\sigma=\nulll$.

\subsubsection{Put}

The $\putt$ operation immediately transitions to the $\seal$ operation as defined
by the following semantics.
\begin{mathpar}
  \inferrule*[Right=Put]{
    \e \rightarrow^{*} \v \\
    \o=\id{\v}
  }{
    \raystep{ \putt(\e) \dbar \S^w}{\sigma, \mu}{ \seal(\o, \v) \dbar \S^w }{\sigma, \mu'}
  }
\end{mathpar}

The $\seal$ operation may be triggered by the main process $\M$ or any of the worker processes $\W_j$,
$j=1, \dots, k$.
An invocation of $\seal$ requires communication with $\S^w$,
which is done over the channel $\alpha_0$ if $\seal$ is invoked from $\M$ and $\alpha_j$ if
$\seal$ is invoked from $\W_j$.
For this reason, we only need to define the parallel semantics of $\seal$ between $\P_i$ and $\S^w$, where
$\P_0 = \M$ and $\P_j = W_j$ for $j=1, \dots, k$.

It is important to note that while processes other than $\P_i$ may be invoking $\seal$,
$S^w$ handles those communications serially. Thus, while the {\bf intermediate}
shared state $\mu$
may be non-deterministic during execution
due to non-deterministic selection of which incoming request to process next,
the {\bf final} shared state $\mu$ is deterministic as all requests
will be processed serially.
The semantics of $\seal$ are defined as follows for $i=0, \dots, k$.
\begin{mathpar}
  \inferrule*[Right=Seal]{
    (\alpha_{i} \, ! \, (\o, \d) => \o) \comarrow{\alpha_{i} \, ! \, (\o, \d)} \o \\
    \comstep{\S^w}{\mu}{\alpha_i \, ? \, (\o, \d)}{\o = \d ; \S^w}{\mu}
  }{
    \comstep{ \seal(\o, \d) \dbar \S^w}{\sigma, \mu}{\lambda}{ \o \dbar \o = \d ; \S^w }{\sigma', \mu}
  }
\end{mathpar}

The Store-Assignment command will transition the resulting program configuration $\mu$ to a configuration $\mu' = \mu[\o=\v]$ if $\d \neq \nulll$, and to $\bot$ otherwise. It is impossible for $\mu$ to have changed after a $\seal$ transition because the $\S^w$ process only lets one $\seal$ through at a time \footnote{A similar $\seal$ operation for commands is defined for remote procedure calls. This is to ensure the $\seal$ operation transitions to the appropriate program configuration when invoked as a command.}.

\subsubsection{Get}
Get may be invoked from two separate process types: The main process and worker processes.
Each process which may invoke $\get$ has a dedicated store process which carries out
the read for that process. Thus, it is sufficient to define the semantics
for a particular process $\P_i$ where $\P_0 = \M$ and $\P_i = \W_j$ for $j = 1, \dots, k$. 
A $\get$ invocation transitions over the following communication configurations before evaluating to $\d$, which may be $\v$ or $\null$.
\begin{enumerate}
\item $\get(\o)$, which submits a request over channel $\gamma_i$. This request is
  received by dedicated store process $\S^r_i$, which is listening for such a request on channel $\gamma_i$.
  This operation always makes progress as each $\P_i$ is able to make at most a single request at a time.
\item $\get(\o)$ transitions to $\rcv(\o)$ on $\P_i$ while the store process $\S^r_i$
  transitions to $\wait(\o)$.
  $\P_i$ cannot make progress until $\o$ becomes available in the object store.
\item $\S^r_i$ transitions to $\snd(\o)$ once the object is available in the object store.
  $\P_i$ makes no progress during this transition.
\item With $\P_i$ in a $\rcv(\o)$ configuration and $\S^r_i$ in a $\snd(\o)$ configuration,
  $\P_i$ is able to transition to $\d$, which is $\nulll$ if $\mu=\bot$, or the value $\mu(\o)=\v$.
  In both cases, $\S^r_i$ transitions to its original listening state.
\end{enumerate}
\begin{mathpar}
  \inferrule*[Right=Get]{
    \xstep{\gamma_{i} \, ! \, \o => \rcv(\o)}{\gamma_{i} \, ! \, \o}{\rcv(\o)} \\
    \op{\S^r_i}{\mu} \comarrow{\gamma_i \, ? \, \o} \op{\sealed(\o) => \gamma_i \, ! \, \mu''(\o) ; \S^r_i}{\mu'}
  }{
    \comstep{\get(\o) \dbar \S}{\sigma, \mu}{\lambda}{\rcv(\o) \dbar \dots \dbar (\wait(\o) ;\S^r_i) \dbar \dots \dbar \S^w}{\sigma', \mu'}
  }
\end{mathpar}
\begin{changemargin}{0.0cm}{0.0cm} 
\begin{mathpar}
  \inferrule*[Right=Wait-True]{
    \comstep{\sealed(\o) => \gamma_i \, ! \, \mu'(\o) ; \S^r_i}{\mu}{\lambda}{\gamma_i \, ! \, \mu'(\o)}{\mu'}
  }{
    \comstep{\rcv(\o) \dbar \dots \dbar (\wait(\o) ; \S^r_i) \dbar \dots \dbar \S^w}{\sigma, \mu}{\lambda}{\rcv(\o) \dbar \dots \dbar (\snd(\o) ; \S^r_i) \dbar \dots \dbar \S^w}{\sigma', \mu'}
  }
\end{mathpar}

\begin{mathpar}
  \inferrule*[Right=Wait-False]{
    \comstep{\sealed(\o) => \gamma_i \, ! \, \mu'(\o) ; \S^r_i}{\mu}{\lambda}{\sealed(\o) => \gamma_i \, ! \, \mu''(\o) ; \S^r_i}{\mu'}
  }{
    \comstep{\rcv(\o) \dbar \dots \dbar (\wait(\o) ; \S^r_i) \dbar \dots \dbar \S^w}{\sigma, \mu}{\lambda}{\rcv(\o) \dbar \dots \dbar (\wait(\o) ; \S^r_i) \dbar \dots \dbar \S^w}{\sigma', \mu'}
  }
\end{mathpar}
\end{changemargin} 

\begin{mathpar}
  \inferrule*[Right=Snd-Rcv]{
    \comstep{\gamma_0 \, ! \, \mu(\o) ; \S^r_0}{\mu}{\gamma_0 \, ! \, \d}{\S^r_0}{\mu'} \\
    \br{\gamma_{0} \, ? \, \x \Rightarrow \x} \comarrow{\gamma_{0} \, ? \, \d} \d
  }{
    \comstep{\rcv(\o) \dbar \dots \dbar (\snd(\o) ; \S^r_i) \dbar \dots \dbar \S^w}{\sigma, \mu}{\lambda}{\d \dbar \S}{\sigma', \mu'}
  }
\end{mathpar}
In the above and in general, $\mu \subseteq \mu' \subseteq \mu''$, which is proven by Lemma \ref{lemma:loseinfo}.

\subsubsection{Remote Function Call}

To simplify the analysis,
we assume function calls are randomly assigned
to workers.
The definition of a remote function call serves only to direct operational
behavior during invocation. Semantics for sampling random numbers and remote function
definitions are given as follows.
\begin{mathpar}
  \inferrule*[Right=Random]{
    \n_2 \sim U(1, ..., \n_1)
  }{
    \raystep{\rand(\n_1)}{\sigma, \mu}{\n_2}{\sigma, \mu}
  }
  \\
  \inferrule*[Right=Remote-Def]{ }{
    \br{\R(\f(\x_1, \dots, \x_m)\{\e\}), (\sigma, \mu)}
  }
\end{mathpar}

Only the main process may invoke a remote function call.
Remote function calls transmit a function definition, as well as a collection of
object ids to a random worker.
Recall that a worker process is defined as follows
\begin{align*}
  \W_i = \dood{ \beta_i \, ? \, (\x_f, \x_r, \x_1, \dots, \x_{m}) \Rightarrow \seal(\x_r, \x_f (\get(\x_1), \dots, \get(\x_{m}))) }
\end{align*}

The worker invokes the provided function and stores the result in the
object store.
Communication between the main process $\M$ and workers $\W_i$
is carried out over the communication channels $\beta_i$, where $i=1, ..., k$.
The semantics of remote function calls need only be defined in parallel for processes $\M$ and $\W$.
\begin{mathpar}
  \inferrule*[Right=R-Call]{
    \sigma(\r) = \R(\f(\x_1, \dots, \x_m) \{ \e \})  \and 
    \o_r = \id{\f, \o_1, \dots, \o_m}  \and 
    i = \rand(k)  \\
    (\beta_i \, ! \, (\f, \o_r, \o_1, \dots, \o_m) => \o_r) \comarrow{\beta_i \, ! \, (\f, \o_r, \o_1, \dots, \o_m)} \o_r \\
    \xstep{\W_i}{\beta_i \, ? \, (\o_f, \o_r, \o_1, \dots, \o_{m})}{ \seal (\o_r, \f (\get(\o_1), \dots, \get(\o_{m})))}
  }{
    \raystep{\r(\o_1, \dots, \o_m) \dbar \W}{\sigma, \mu}{\o_r \dbar \dots  \dbar \seal (\o_r, \f (\get(\o_1), \dots, \get(\o_{m}))) ; \W_i  \dbar \dots}{\sigma', \mu'}
  }
\end{mathpar}

The following seal command for worker processes transitions the program to its final state
by evaluating all $\get$ operations, evaluating the function,
and actually invoking $\seal$ on the resulting value.
\begin{mathpar}
  \inferrule*[Right=Seal-Cmd]{
    \f(\d_1, \dots, \d_m) \rightarrow^{*} \d \\
    (\alpha_{i} \, ! \, (\o, \d) => \o) \comarrow{\alpha_{i} \, ! \, (\o, \d)} \o \\
    \comstep{\S^w}{\mu}{\alpha_i \, ? \, (\o, \d)}{\o = \d ; \S^w}{\mu}
  }{
    \comstep{ \seal(\o, \f(\d_1, \dots, \d_m)) \dbar \S^w}{\sigma, \mu}{\lambda}{ \skipp \dbar \o = \d ; \S^w }{\sigma', \mu}
  }
\end{mathpar}
