# Supplementary material for: NumS: Scalable Array Programming for the Cloud
Source: arXiv:2206.14276 source file (2022-07-13)
Supplement: Supplementary file 5 [file 040-translation.tex]

\section{Parallelization of Serial Python Programs}
\label{appendix:translation}

Let $\T$ denote the translation operator,
which is inductively defined as follows.
\begin{align*}
% Commands
\T(\skipp) & \equiv \skipp \\
\T(\c_1 ; \c_2) & \equiv (\T(\c_1); \T(\c_2)) \\
\T(\x = \e) & \equiv \x = \T(\e) \\
\T(\iif{\b}{\c_1}{\c_2}) & \equiv \iif{\get(\T(\b))}{\T(\c_1)}{\T(\c_2)} \\ 
\T(\while{\b}{\c}) & \equiv \while{\get(\T(\b))}{\T(\c)} \\ 
% Functions
\T(\f(\x_1, \dots, \x_m)\{\e\}) & \equiv \R(\f(\x_1, \dots, \x_m)\{\e\}) \\
\T(\f(\e_1, \dots, \e_m)) & \equiv \R(\f)(\T(\e_1), \dots, \T(\e_m)) \\
\T(\R(\f)) & \equiv \R(\f) \\
% Unary Operations
\T(-\a) & \equiv \R(-)(\T(\a)) \\
\T(\nott \b) & \equiv \R(\nott)(\T(\b)) \\
% Binary Operations
\T(\a_1 \bop_2 \a_2) & \equiv \R(\bop_2)(\T(\a_1), \T(\a_2)) \\
\T(\b_1 \bop_2 \b_2) & \equiv \R(\bop_2)(\T(\b_1), \T(\b_2)) \\
\T(\v) & \equiv \putt(\v) \\
\T(\x) & \equiv \x \\
\end{align*}
In the above, $\bop_2$ is shorthand for arbitrary binary operations 
conditioned on the operands. For instance, $\bop_2$ in $\a_1 \bop_2 \a_2$ stands for all
binary arithmetic operations.
$\R(\bop_2)$ is the remote function which takes two arguments and returns the result of applying $\bop_2$ on those arguments.
In general, for an $\n$-ary operation $\bop_{\n}$,
$\R(\bop_{\n})$ is the remote function which takes $\n$ arguments and returns the result of applying the $\n$-ary operation.
% The blue text denotes concrete if-then-else and while Python statements.

% With this translation operator in hand, we translate programs $\c$ into
% Futures programs, execute them, and iterate
% over the resulting set of variables in $\sigma$,
% and replace them with their values by invoking $\get$ on the object id they map to.
% Formally, for some program $\c$, we obtain the main Futures program $\M$ as follows.
% \begin{align}
% \M = \T(\c) ; (\forall \x, \o \in \sigma. \, \x = \get(\o))
% \end{align}

% \subsection{Example}
% Consider the following program, which we denote by $\c$.
% \begin{lstlisting}
% x = lambda n: n + n
% y = 0
% z = 2
% w = x(20)
% v = w + y + z
% \end{lstlisting}

% The corresponding Futures program $\T(\c)$ is the following.
% \begin{lstlisting}
% x = R(lambda n: n + n)
% y = put(0)
% z = put(2)
% w = x(put(20))
% v = R(lambda *x: sum(x))(w, y, z)
% \end{lstlisting}
