# Supplementary material for: NumS: Scalable Array Programming for the Cloud
Source: arXiv:2206.14276 source file (2022-07-13)
Supplement: Supplementary file 6 [file 050-proofs.tex]

\section{Correctness Proofs}
\label{appendix:proofs}

The notion of correctness of translated programs is captured
by the following theorem.
\begin{equation}
\label{maintheorem}
\begin{aligned}
  \textbf{if } & \op{\c}{\sigma} \rightarrow^{*} \sigma ' \textbf{ and } \sigma' \neq \bot \\
  \textbf{then } & \rayop{\T(\c)}{\W}{\S}{\sigma, \mu} \rightarrow^{*} \rayop{\skipp}{\W}{\S}{\sigma'', \mu'}  \\
  \textbf{such that } & \forall (\x, \v) \in \sigma'. \, (\sigma''(\x), \v) \in \mu'.
\end{aligned}
\end{equation}
Note that in this theorem we assume $\c$ is terminating.
We deal with the case of non-terminating programs in Lemma \ref{lemma:nonterm}.
We need to prove this for all Sub-Python commands,
so we proceed by structural
induction on the derivation of Sub-Python commands and Sub-Futures commands.
Specifically, these are the Sub-Futures operation transitions, as well as the resulting
configuration transitions, that appear in translated Sub-Python programs.
In our proofs, we make the following simplifying assumptions:
\begin{enumerate}
  \item The number of worker processes $k=1$.
\end{enumerate}

\subsection{Remark: Object Hashes are Unique}
The function $\id{\cdot}$ generates a hash of its input.
For any function $\f(\x_1 \dots, \x_m)\{ \e \}$
the identifier $\o = \id{\f, \o_1, \dots, \o_m}$ uniquely identifies the invocation of $\f$
on $\v_1, \dots, \v_m$ where $\o_i = \id{\v_i}$.
This is trivially true as the expressions $\e$ are deterministic.
If an expression is non-terminating, the entire context in which the expression occurs
transitions to $\nulll$.

\subsection{Lemma: Object Store Does Not Lose Information}
\label{lemma:loseinfo}

Some of the following proofs require that concurrent write requests
sent to $\S^w$ from $\M$ and the $\W_j$ never result in a configuration whereby
the store loses previously written information.
We only care about the case where expressions evaluate to values.
We deal with the non-terminating case in Lemma \ref{lemma:nonterm}.
% Let $\V_i \equv \d_{i,0}, \dots, \d_{i, m_i}$. Then
Formally,
\begin{align*}
  & \textbf{if } \rayop{\putt(\v_0)}{\putt(\v_1) \dbar \dots \dbar \putt(\v_k)}{\S^w}{\sigma, \mu} \rightarrow^{*} \rayop{\skipp}{\W}{\S}{\sigma, \mu'} \\
  & \textbf{then } \forall \, i=0, \dots, k \, . \, (\id{\v_i}, \v_i) \in \mu'.
\end{align*}

Consider the process $\S^w$, which can be in one of two configurations:
$\S^w$, or $\o_i = \v_i ; \S^w$. In the configuration $\S^w$, the summation over incoming messages
non-determinisitcally accepts a single message from the incoming messages over channels $\alpha_i$.
This transition yields the configuration $\o_i = \v_i ; \S^w$. Since $\S^w$ is the only process
listening on channels $\alpha_0, \dots, \alpha_k$, other processes $P_j$ where $j \neq i$
are blocking until $\o_i = \v_i ; \S^w \rightarrow \S^w$, at which point $\mu[\o_i = \v_i]$,
and the next incoming write request will be written to $\mu[\o_i = \v_i]$.
Thus, the cardinality of the store $\mu$ is monotonically increasing,
and $\mu$ does not lose previously written information. \qed

\subsection{Correctness of Translated Expressions}
We start by proving correctness
of all translated expressions $\e$.
The translation of an expression $\e$ is simply $\T(\e)$.
We need to prove the following.
\begin{equation*}
  \textbf{if } (\e \rightarrow^{*} \v) \textbf{ then } \rayop{\T(\e)}{\W}{\S}{\sigma, \mu} \rightarrow^{*} \rayop{\o}{\W}{\S}{\sigma, \mu'} \textbf{ such that } (\o, \v) \in \mu.
\end{equation*}
We proceed by structural induction on the derivation of expressions.

\subsubsection{Base Case}
Our base cases are the following:
\begin{enumerate}
  \item $\e \equiv \v$. We have $\T(\v) = \putt(\v)$.
  \item $\e \equiv \x$. This follows immediately from $\e = \v$ since $\T(\x) = \x$ and $\sigma(\T(\x))$ will be an object id by definition of the translation operator.
\end{enumerate}
$\putt(\v)$ provides a derivation of the step to $\seal(\o, \v)$,
and the derivation of $\seal$  yields
$$\rayop{\seal(\o, \v)}{\W}{\S}{\sigma, \mu} \comarrow{\lambda} \rayop{\o}{\W}{\S^r \dbar \o=\v; \S^w}{\sigma, \mu}.$$

The proof for the base case follows immediately from the derivation of $\o=\v$:
$$\rayop{\o}{\W}{\S^r \dbar \o=\v; \S^w}{\sigma, \mu} \rightarrow \rayop{\o}{\W}{\S}{\sigma, \mu[\o=\v]}.$$

\subsubsection{Functions}
The rest of expressions follow immediately from a proof of function invocation,
as the binary operations of arithmetic and boolean expressions, such as $a_1 + a_2$,
are translated to remote functions $\R(+)(\putt(a_1), \putt(a_2))$, where $\R(+) \equiv \R(\f(\x_1, \x_2)\{ \x_1 + \x_2 \})$. We must show that 
\begin{align*}
  \textbf{if } & (\f(\v_1, \dots, \v_m) \rightarrow \v) \\
  \textbf{ then } & \rayop{\T(\f(\v_1, \dots, \v_m))}{\W}{\S}{\sigma, \mu}
  \rightarrow^{*}
  \rayop{\o}{\W}{\S}{\sigma, \mu'} \\
  \textbf{ such that } & (\o, \v) \in \mu'.
\end{align*}

$\T(\f(\v_1, \dots, \v_m)) \equiv \R(\f)(\T(\v_1), \dots, \T(\v_m))$.
By the induction hypothesis, we have that $\T(\v_i) \equiv \putt(\v_i) \rightarrow^{*} \o_i$,
and that by Lemma \ref{lemma:loseinfo}, the entire program will transition to a configuration
$$\rayop{\R(\f)(\o_1, \dots, \o_m)}{\W}{\S}{\sigma, \mu''},$$

where $\forall \, i=1, \dots, m . \, (\o_i, \v_i) \in \mu''$.
The rule for remote function call provides a derivation of the transition
to $$\rayop{\o}{\seal(\o, \f(\get(\o_1), \dots, \get(\o_m)));W_1}{\S}{\sigma, \mu''}.$$

For $\get(\o_1)$, the derivation of $\get$ provides the
following transition:
\begin{align*}
  & \rayop{\o}{\seal(\o, \f(\get(\o_1), \dots, \get(\o_m)));\W_1}{\S}{\sigma, \mu''} \\
  \comarrow{\lambda} &
  \rayop{\o}{\seal(\o, \f(\rcv(\o_1), \dots, \get(\o_m)));\W_1}{(\wait(\o_1);\S^r_0) \dbar \S^w}{\sigma, \mu''}.
\end{align*}

For $\wait$ to make progress, $\sealed(\o_1)$ must evaluate to $\true$.
The derivation of $\sealed(\o_1)$ requires that $\exists \, \v \, . \, (\o_1, \v) \in \mu''$.
This is satisfied since $\mu''(\o_1) = \v_1$. Thus, the derivation of $\wait$ provides the
remaining transitions:
\begin{align*}
  & \rayop{\o}{\seal(\o, \f(\rcv(\o_1), \dots, \get(\o_m)));\W_1}{(\wait(\o_1);\S^r_0) \dbar \S^w}{\sigma, \mu''} \\
  \comarrow{\lambda} &
  \rayop{\o}{\seal(\o, \f(\rcv(\o_1), \dots, \get(\o_m)));\W_1}{(\snd(\o_1);\S^r_0) \dbar \S^w}{\sigma, \mu''} \\
  \comarrow{\lambda} &
  \rayop{\o}{\seal(\o, \f(\v_1, \dots, \get(\o_m)));\W_1}{\S}{\sigma, \mu''}.
\end{align*}

The same holds for the remaining $\get$ operations, which 
evaluate left-to-right as specified by the evaluation order of
function arguments and 
yield $\rayop{\o}{\seal(\o, \f(\v_1, \dots, \v_m))}{\S}{\sigma, \mu''}.$
Function evaluation yields $\rayop{\o}{\seal(\o, \v);\W_1}{\S}{\sigma, \mu''},$
and finally the $\seal$ operation yields the following sequence of configurations
% Seal, the command, transitions to skip.
\begin{align*}
  & \rayop{\o}{\seal(\o, \v);\W_1}{\S}{\sigma, \mu''} \\
  \comarrow{\lambda} &
  \rayop{\o}{\skipp;\W_1}{\S^r \dbar \o = \v ; \S^w}{\sigma, \mu''} \\
  \comarrow{\lambda} &
  \rayop{\o}{\W}{\S}{\sigma, \mu''[\o = \v]}.
\end{align*}

This concludes the proof for expressions. \qed

\subsection{Lemma: Get is Correct}
\label{lemma:get}
We want to show that if $\e \rightarrow^{*} \v$ then $\get(\T(\e)) \rightarrow^{*} \v$.
We know that $\T(\e)) \rightarrow^{*} \o$ yields a state $\mu'(o) = \v$ from the proof of correctness of expressions.
For $\get(\o)$, the derivation of $\get$ provides the
following transitions:
\begin{align*}
  & \rayop{\get(\o)}{\W}{\S}{\sigma, \mu'} \\
  \comarrow{\lambda} & \rayop{\rcv(\o)}{\W}{(\wait(\o);\S^r_0) \dbar \S^w}{\sigma, \mu'} \\
  \comarrow{\lambda} & \rayop{\rcv(\o)}{\W}{(\snd(\o);\S^r_0) \dbar \S^w}{\sigma, \mu'} \\
  \comarrow{\lambda} & \rayop{\v}{\W}{\S}{\sigma, \mu'}.
\end{align*}
To make progress, $\wait(\o)$ requires that $\sealed(\o)$ evaluates to $\true$,
and we have by I.H. $\exists \, \v \, . \, (\o, \v) \in \mu'$.

\subsection{Correctness of Translated Commands}

\subsubsection{Assignment}
$\c \equiv \x = \e$. We have $\T(\x = \e) \equiv \x = \T(\e)$.
We have $\br{\x = \e, \sigma} \rightarrow^{*} \br{\v, \sigma'}$.
By definition of the operator $\T$ and the induction hypothesis,
we have $\M \equiv \x = \o$ and $\mu'$ such that $\mu'(\o) = \v$.
Assignment yields $\rayop{\x=\o}{\W}{\S}{\sigma, \mu'} \rightarrow \rayop{\skipp}{\W}{\S}{\sigma'', \mu'}$ where $\sigma'' = \sigma[\x=\o]$. Thus, we have $(\x, \v) \in \sigma'$ and $(\sigma''(\x), \v) \in \mu'$.

\subsubsection{Sequence}
$\c \equiv \c_1; \c_2$.
Let $\sigma_0'$ be the intermediate state after executing $\c_1$ and before executing $\c_2$,
and $\sigma_0''$ be the intermediate state after executing $T(\c_1)$ and before executing $T(\c_2)$.
By induction hypothesis, for $\c_1$ we have $\forall (\x, \v) \in \sigma_1'. \, (\sigma_1''(\x), \v) \in \mu_1'$.
By induction hypothesis, for $\c_2$ we have $\forall (\x, \v) \in \sigma_2'. \, (\sigma_2''(\x), \v) \in \mu_2'$.
By definition of the sequence command, we have $\sigma_0' = \sigma_1'$, $\sigma_0'' = \sigma_1''$.
Thus, $\sigma' = \sigma_2'$, $\sigma'' = \sigma_2''$, $\mu' = \mu_2'$,
and $\forall (\x, \v) \in \sigma'. \, (\sigma''(\x), \v) \in \mu'$.

\subsubsection{If-Then-Else}
$\c \equiv \iif{\b}{\c_1}{\c_2}$.
We have by the I.H. and Lemma \ref{lemma:get} that $\b = \get(\T(b))$.
Thus, if $\b = \get(\T(\b)) = \true$ then by I.H. the theorem holds for
$\c_1$. Likewise, $\b = \get(\T(\b)) = \false$, the theorem holds for $\c_2$
by I.H.

\subsubsection{While Loops}
Note here we only prove the terminating case.
We prove the non-terminating cases in Lemma \ref{lemma:nonterm}, 
where $\br{\while{\b}{\c}, \sigma} \rightarrow \br{\skipp, \bot}$,
and in such cases we have that $\mu$ also transitions to $\bot$.
We want to show Theorem \ref{maintheorem} for $\c \equiv \while{\b}{\c'}$.

By I.H. and Lemma \ref{lemma:get},
if $\br{\b, \sigma} \rightarrow^{*} \br{\true, \sigma}$
then $\br{\get(\T(\b)), \sigma, \mu} \rightarrow^{*} \br{\true, \sigma, \mu'}$.
The same holds when $\b$ evaluates to $\false$. 
If $\b$ evaluates to $\false$, so does $\get(\T(\b))$, which means $\sigma = \sigma ' = \sigma ''$ and $\mu = \mu'$, proving the result for $\false$.
If $\b$ evaluates to $\true$, then 
$$\br{\while{\get(\T(\b))}{\T(\c')}, \sigma, \mu} \rightarrow \br{\T(\c') ; \while{\get(\T(\b))}{\T(\c')}, \sigma, \mu}.$$
We have already proven the theorem for sequence,
thus, we know that if $\c'$ and $\T(\c')$ execute $k$ times and terminate in state
$\sigma'$ and $(\sigma'', \mu')$, respectively, then $\forall (\x, \v) \in \sigma'$,
$(\sigma''(\x), \v) \in \mu'$.

We now want to show that if the serial loop body $\c'$ executes $k$ times,
the parallel loop body $\T(\c')$ also executes $k$ times.
We show this by proving that $\b = \get(\T(\b))$ after every loop iteration.
We have this result by the I.H. for $k=1$. We can prove the theorem
for arbitrary $k$ by showing that the theorem holds after 
executing $\c'$.
Let $\br{\c', \sigma_0} \rightarrow^{*} \br{\skipp, \sigma_0'}$
and $\br{\T(\c'), \sigma_0} \rightarrow^{*} \br{\skipp, \sigma_0'', \mu_0'}$. 
We have by the I.H. that $\forall (\x, \v) \in \sigma_0'. \, (\sigma_0''(\x), \v) \in \mu_0'$. Thus, after the $k$th execution of $\c'$ and $\T(\c')$, 
we have again by the I.H. and Lemma \ref{lemma:get} that 
if $\br{\b, \sigma_0'} \rightarrow^{*} \br{\true, \sigma_0'}$
then $\br{\get(\T(\b)), \sigma_0'', \mu_0'} \rightarrow^{*} \br{\true, \sigma_0'', \mu_0''}$.
The same holds when $\b$ evaluates to $\false$. 
This concludes the proof of correctness for translated programs that terminate. \qed

\subsection{Corollary: Non-Terminating Programs Translate to Non-Terminating Programs}
\label{lemma:nonterm}
To show that non-terminating
Sub-Python programs are translated to non-terminating Sub-Futures programs,
we need to prove the following corollary for expressions and while loops.

\begin{equation}
    \label{theorem:nonterm}
    \begin{aligned}
      \textbf{if } & \op{\c}{\sigma} \rightarrow^{*} \op{\skipp}{\bot} \\
      \textbf{then } & \rayop{\T(\c)}{\W}{\S}{\sigma, \mu} \rightarrow^{*} \rayop{\skipp}{\W}{\S}{\bot, \bot}
    \end{aligned}
\end{equation}

\subsubsection{Expressions}
Here we want to show that, for some non-terminating expression $\e$,
\begin{align*}
  \textbf{if } & \op{\e}{\sigma} \rightarrow^{*} \op{\nulll}{\bot} \\
  \textbf{then } & \rayop{\T(\e)}{\W}{\S}{\sigma, \mu} \rightarrow^{*} \rayop{\o}{\W}{\S}{\bot, \bot}
\end{align*}
The only relevant case is when $\e = \f(\v_1, \dots, \v_m)$, and in such cases, $\T(\f(\v_1, \dots, \v_m))$ is a remote function. Let $\r(\o_1, \dots, \o_m) = \T(\f(\v_1, \dots, \v_m))$.
By the derivation of remote function calls, on worker $i$
we transition to a $\seal$ operation
of the form $\seal(\o, \f(\v_1, \dots, \v_m))$ and yield the object id $\o$ corresponding to the result of executing $\f$ \footnote{A $\get$ invocation on such an object id will yield $\nulll$. This is not needed in the proof but is worth noting.}.
The derivation of $\seal$ relies on the evaluation of $\f$, which we know evaluates to $\nulll$. Thus, the $\seal$ command transitions to a state where 
$\S^w \equiv \o = \nulll; \S^w$. The derivation of $Store-Assign-\infty$ handles
this state by transitioning $\mu$ to $\bot$.
The derivations for Parallel-Store-Error and Parallel-Store-Error-2
handle this state by transitioning $\sigma$ to $\bot$, and the main process to $\skipp$.
This proves the theorem for expressions and shows that
whenever we translate a non-terminating recursive function,
the translated remote function is also non-terminating and handled appropriately.

\subsubsection{While Loops}
We now prove Theorem \ref{theorem:nonterm} for $\c \equiv \while{\b}{\c'}$, which is the only command that may not terminate. By the derivation of While-$\infty$, if $\while{\b}{\c'}$ is non-terminating, we have $\br{\while{\b}{\c'}, \sigma} \rightarrow \br{\skipp, \bot}$,
which relies on the premise $$\forall k. \, \br{\whilek{k}{\b}{\c'}, \sigma} \rightarrow \br{\skipp, \bot}.$$
If we prove that this premise is preserved under the translation operator, then
we have proven our result.
We want to prove that
\begin{align*}
  \textbf{if } & \forall k_1. \, \br{\whilek{k_1}{\b}{\c'}, \sigma} \rightarrow^{k_1+1} \br{\skipp, \bot} \\
  \textbf{then } & \forall k_2. \, \rayop{\whilek{k_2}{\get(\T(\b))}{\T(\c')}}{\W}{\S}{\sigma, \mu} \rightarrow^{k_2+1} \rayop{\skipp}{\W}{\S}{\bot, \bot},
\end{align*}
We proceed by induction on $k_2$.
If $k_2=0$, then by Theorem \ref{maintheorem} we have that $\br{\get(\T(\b)), \sigma, \mu}$ evaluates to the same value as $\br{\b, \sigma}$. 
Since $\br{\b, \sigma}$ evaluates to $\true$ for all $k_1$,
$$\rayop{\whilek{0}{\get(\T(\b))}{\T(\c')}}{\W}{\S}{\sigma, \mu} \rightarrow^{1} \rayop{\skipp}{\W}{\S}{\bot, \mu}.$$ By the derivation of Parallel-Main-Error and Parallel-Main-Error-2, the Sub-Futures program transitions to 
a state where $\mu = \bot$.

For $k_2 > 0$, 
% we have that $\forall k_1. \, \br{\whilek{k_1}{\b}{\c'}, \sigma} \rightarrow^{k_1+1} \br{\skipp, \bot}$. 
% The derivation of While-k-True provides the transition 
% $\br{\whilek{k_1}{\b}{\c'}, \sigma} \rightarrow^{1} \br{\c' ; \whilek{k_1-1}{\b}{\c'}, \sigma}$.
we'll show that 
$$\br{\whilek{k_2}{\get(\T(\b))}{\T(\c')}, \sigma, \mu} \rightarrow^{1} \br{\T(\c') ; \whilek{k_2-1}{\get(\T(\b))}{\T(\c')}, \sigma, \mu'}.$$
The derivation of While-k-True provides the transition 
$\br{\whilek{k}{\b}{\c'}, \sigma} \rightarrow^{1} \br{\c' ; \whilek{k-1}{\b}{\c'}, \sigma}$ and requires that $\b$ evaluates to $\true$.
By theorem \ref{maintheorem} and Lemma \ref{lemma:get} we have that if $\br{\b, \sigma}$ evaluates to $\true$, then $\br{\get(\T(\b)), \sigma, \mu}$ must also evaluate to $\true$.
Since $\b$ evaluates to $\true$ for all $k_1$, 
$\br{\whilek{k_2}{\get(\T(\b))}{\T(\c')}, \sigma, \mu}$
$\rightarrow$
$\br{\T(\c') ; \whilek{k_2-1}{\get(\T(\b))}{\T(\c')}, \sigma, \mu'}$.
The derivation of sequence yields the transition
$$\br{\T(\c') ; \whilek{k_2-1}{\get(\T(\b))}{\T(\c')}, \sigma, \mu'} \rightarrow 
\br{\whilek{k_2-1}{\get(\T(\b))}{\T(\c')}, \sigma', \mu''}.$$
By the I.H., we have that 
$\br{\whilek{k_2-1}{\get(\T(\b))}{\T(\c')}, \sigma', \mu''} \rightarrow^{k_2} \rayop{\skipp}{\W}{\S}{\bot, \bot}.$ \qed
