# Supplementary material for: NumS: Scalable Array Programming for the Cloud
Source: arXiv:2206.14276 source file (2022-07-13)
Supplement: Supplementary file 7 [file 060-arrays.tex]

\section{Arrays}
\label{appendix:arrays}

We now extend our language to support 2-dimensional arrays
and basic linear algebra operations.
Our syntax, semantics, and translation operators are defined 
for a core subset of the NumPy API, which illustrates our general approach
to translating NumPy syntax to our representation of multi-dimensional futures
and their operations. The definition of Assignment differs slightly 
from what we implement in practice.

\subsection{Syntax}

\begin{align*}
\c \enspace \Coloneqq & \enspace ... \sbar \x[\ii_1:\ii_2 , \mathbf{j}_1:\mathbf{j}_2] = \e \sbar \x[\ii, :] = \e \sbar \x[:, \mathbf{j}] = \e \sbar \x[\ii, \mathbf{j}] = \e \\
\e \enspace \Coloneqq & \enspace ... \sbar \A \\
\A \enspace \Coloneqq & \enspace \N(\n, \mathbf{m}) \sbar \x \\ 
& \sbar \Zeros(\n, \mathbf{m}) \sbar \Read(\s, \n, \mathbf{m}) \sbar \Read(\s, \ii_1:\ii_2, \mathbf{j}_1:\mathbf{j}_2) \\ 
& \sbar \A[\ii_1:\ii_2, \mathbf{j}_1:\mathbf{j}_2] \sbar \A[\ii, :] \sbar \A[:, \mathbf{j}] \sbar \A[\ii, \mathbf{j}] \\
& \sbar \A.\T \sbar \A_1 @ \A_2 \sbar \A_1 + \A_2 \sbar \A_1 - \A_2 \\
& \sbar \A * \a \sbar \A + \a \sbar \A - \a \sbar \A / \a \\
\a \enspace \Coloneqq & \enspace ... \sbar \A.\shape[0] \sbar \A.\shape[1] \sbar \pow(\x, \n) \sbar \mathbf{sqrt}(\n) \sbar \norm(\A_1, \A_2) \\
\v \enspace \Coloneqq & \enspace ... \sbar \N(\n, \mathbf{m})
\end{align*}

\iffalse
\begin{verbatim}
c ::= ... | x[i_1:i_2, j_1:j_2] = e | x[i, :] = e | x[:, j] = e | x[i, j] = e 
e ::= ... | A
A ::= N(n, m) | x 
    | Zeros(n, m) | Read(s, n, m) | Read(s, i_1:i_2, j_1:j_2) 
    | A[i_1:i_2, j_1:j_2] | A[i, :] | A[:, j] | A[i, j]
    | A.T | A_1 @ A_2 | A_1 + A_2 | A_1 - A_2 
    | A * a | A + a | A - a | A / a
a ::= ... | A.shape[0] | A.shape[1] | pow(x, n) | sqrt(n) | norm(A_1, A_2)
v ::= ... | N(n, m)
\end{verbatim}
\fi

We have $\A \in \mathcal{A}$, where $\mathcal{A}$ is the set 
defined above in BNF form, and $\N(n, m) \in \mathbb{R}^{n \times m}$ is a
real-valued 2-dimensional array.
$\Zeros$ and $\Read$ are the only constructors for real-valued arrays.
We introduce $\omega \subseteq \mathcal{S} \times \mathbb{N} \times \mathbb{N} \times \mathbb{R}$, which corresponds to a read-only object containing entries of 2-dimensional arrays.
We access entries using $\omega(\s, \n_1, \n_2) \in \mathbb{R}$. $\s \in \mathcal{S}$ and $\mathcal{S}$ corresponds to the space of all strings. For brevity, we exclude $\omega$ in program configurations.

\subsection{Semantics}

\subsubsection{Declaration}
\begin{mathpar}
  \inferrule*[Right=Zeros]{
    0 < n, m \and
    0 \leq i < n \and 
    0 \leq j < m \and 
    \N(n, m)[i, j] = 0
  }{
    \br{\Zeros(n, m), \sigma} \rightarrow \br{\N(n, m), \sigma}
  }
  \\
  \inferrule*[Right=Read]{
    0 < n, m \and
    0 \leq i < n \and 
    0 \leq j < m \and 
    \N(n, m) = \Read(\s, \, 0:n, \, 0:m)
  }{
    \br{\Read(\s, n, m), \sigma} \rightarrow \br{\N(n, m), \sigma}
  }
  \\
  \inferrule*[Right=Read-Block]{
    n = i_2-i_1 \and
    m = j_2-j_1 \and
    0 < n, m \and
    i_1 \leq i < i_2 \and 
    j_1 \leq j < j_2 
    \\
    (\s,\, n-1,\, m-1) \in \omega \and
    \N(n, m)[i, j] = \omega(\s, i, j)
  }{
    \br{\Read(\s,\, i_1:i_2,\, j_1:j_2), \sigma} \rightarrow \br{\N(n, m), \sigma}
  }
  \\
  \inferrule*[Right=Array-Lookup]{
  \sigma(x) = \N(n, m)
  }{
    \br{\x, \sigma} \rightarrow \br{\N(n, m), \sigma}
  }
\end{mathpar}

\subsubsection{Selection}
Selection \\

\resizebox{0.9\textwidth}{!}{%
\centering
\begin{mathpar}
  \inferrule*[Right=Select-Block]{
  \br{\A, \sigma} \rightarrow \br{\N'(n', m'), \sigma} \and
    0 \leq i_1 < i_2 \leq n' \and 
    0 \leq j_1 < j_2 \leq m' 
    \\
    n = i_2-i_1 \and
    m = j_2-j_1 \and
    0 < n, m \and
    0 \leq i < n \and 
    0 \leq j < m 
    \\
    \N(n, m)[i, j] = \N'(n', m')[i_1 + i, j_1 + j]
  }{
    \br{\A[i_1:i_2, \, j_1:j_2], \sigma} \rightarrow \br{\N(n, m), \sigma}
  }
  \\
  \inferrule*[Right=Select-Row]{
    \br{\A, \sigma} \rightarrow \br{\N'(n, m), \sigma}
    \\
    0 \leq i < n \and
    \br{\N'(n, m)[i:i+1, \, 0:m], \sigma} \rightarrow \br{\N(1, m), \sigma}
  }{
    \br{\A[i, :], \sigma} \rightarrow \br{\N(1, m), \sigma}
  }
  \\
  \inferrule*[Right=Select-Col]{
    \br{\A, \sigma} \rightarrow \br{\N'(n, m), \sigma}
    \\
    0 \leq j < m \and
    \br{\N'(n, m)[0:n, \, j:j+1], \sigma} \rightarrow \br{\N(n, 1), \sigma}
  }{
    \br{\A[:, j], \sigma} \rightarrow \br{\N(n, 1), \sigma}
  }
  \\
  \inferrule*[Right=Select-Entry]{
    \br{\A, \sigma} \rightarrow \br{\N'(n, m), \sigma} \and
    0 \leq i < m \and
    0 \leq j < m \\\
    \br{\N'(n, m)[i:i+1, \, j:j+1], \sigma} \rightarrow \br{\N(1, 1), \sigma} \and
    % \n = \N(1, 1)[0, 0]
  }{
    \br{\A[i, j], \sigma} \rightarrow \br{\N(1, 1), \sigma}
  }
\end{mathpar}
}

\subsubsection{Array Assignment}
We model array assignments as pure functions: Assigning new values to entries of an existing array produces a new array object.
% Some work needs to be done to make sure entry assignment 
% goes through when $\e$ evaluates to a real.

\resizebox{0.9\textwidth}{!}{%
\centering
\begin{mathpar}
  \inferrule*[Right=Assign-Block]{
    \br{\x, \sigma} \rightarrow \br{\N'(n', m'), \sigma} \and
    0 \leq i_1 < i_2 \leq n' \and 
    0 \leq j_1 < j_2 \leq m' \and
    \\
    \br{\e, \sigma} \rightarrow \br{\N''(n'', m''), \sigma} \and
    n'' = i_2-i_1 \and
    m'' = j_2-j_1
    \\
    0 \leq i'' < n'' \and 
    0 \leq j'' < m'' \and 
    0 \leq i' < n' \wedge i' \neq i'' \and 
    0 \leq j' < m' \wedge j' \neq j'' \and
    \\
    n = n' \and
    m = m'
    \\
    \N(n, m)[i_1 + i'', j_1 + j''] = \N''(n'', m'')[i'', j''] \and
    \N(n, m)[i', j'] = \N'(n', m')[i', j']
  }{
    \br{\x[i_1:i_2, \, j_1:j_2] = \e, \sigma} \rightarrow \br{\N(n, m), \sigma}
  }
  \\
  \inferrule*[Right=Assign-Row]{
    \br{\x, \sigma} \rightarrow \br{\N'(n, m), \sigma} \and
    i_1 = i \and i_2 = i+1 \and j_1 = 0 \and j_2 = m \\
    \br{\x[i_1:i_2, \, j_1:j_2] = \e, \sigma} \rightarrow \br{\N(n, m), \sigma}
  }{
    \br{\x[i, :] = \e, \sigma} \rightarrow \br{\N(n, m), \sigma}
  }
  \\
  \inferrule*[Right=Assign-Col]{
    \br{\x, \sigma} \rightarrow \br{\N'(n, m), \sigma} \and
    i_1 = 0 \and i_2 = n \and j_1 = j \and j_2 = j+1 \\
    \br{\x[i_1:i_2, \, j_1:j_2] = \e, \sigma} \rightarrow \br{\N(n, m), \sigma}
  }{
    \br{\x[:, j] = \e, \sigma} \rightarrow \br{\N(n, m), \sigma}
  }
  \\
  \inferrule*[Right=Assign-Entry]{
    \br{\x, \sigma} \rightarrow \br{\N'(n, m), \sigma} \and
    i_1 = i \and i_2 = i+1 \and j_1 = j \and j_2 = j+1 \\
    \br{\x[i_1:i_2, \, j_1:j_2] = \e, \sigma} \rightarrow \br{\N(n, m), \sigma}
  }{
    \br{\x[i, j] = \e, \sigma} \rightarrow \br{\N(n, m), \sigma}
  }
\end{mathpar}
}

\subsubsection{Operators}
We rely on underlying implementations of array operators, such as the $\mm$
operator implemented by NumPy \cite{numpy}. We denote such reliance
by coloring the operator blue. We denote the binary operations
corresponding to Array-Array operators, and Array-Real operators
as $\bop$.

\begin{mathpar}
  \inferrule*[Right=Transpose]{
    \br{\A, \sigma} \rightarrow \br{\N'(n, m), \sigma}
    \\
    0 \leq i < n \and 
    0 \leq j < m \and
    \N(m, n)[j, i] = \N'(n, m)[i, j]
  }{
    \br{\A.\top, \sigma} \rightarrow \br{\N(m, n), \sigma}
  }
  \\
  \inferrule*[Right=Matrix-Multiply]{
    \br{\A_1, \sigma} \rightarrow \br{\N_1(n_1, m_1), \sigma} \and
    \br{\A_2, \sigma} \rightarrow \br{\N_2(n_2, m_2), \sigma}
    \\
    m_1 = n_2 \and
    n = n_1 \and
    m = m_2 \and
    \N(n, m) = \N_1(n_1, m_1) \bmm \N_2(n_2, m_2)
  }{
    \br{\A_1 \mm \A_2, \sigma} \rightarrow \br{\N(n, m), \sigma}
  }
  \\
  \inferrule*[Right=Array-Array-Binary-Op]{
    \br{\A_1, \sigma} \rightarrow \br{\N_1(n_1, m_1), \sigma} \and
    \br{\A_2, \sigma} \rightarrow \br{\N_2(n_2, m_2), \sigma}
    \\
    n = n_1 = n_2 \and
    m = m_1 = m_2 \and
    \N(n, m) = \N_1(n_1, m_1) \bbf{ $\bop$ } \N_2(n_2, m_2)
  }{
    \br{\A_1 \bop \A_2, \sigma} \rightarrow \br{\N(n, m), \sigma}
  }
  \\
  \inferrule*[Right=Array-Real-Binary-Op]{
    \br{\A, \sigma} \rightarrow \br{\N'(n, m), \sigma} \\
    \br{\a, \sigma} \rightarrow \br{\n, \sigma} \\
    \N(n, m) = \N'(n, m) \bbf{ $\bop$ } \n
  }{
    \br{\A \bop \a, \sigma} \rightarrow \br{\N(n, m), \sigma}
  }
\end{mathpar}

\subsubsection{Additional Array and Arithmetic Expressions}

\begin{mathpar}
  \inferrule*[Right=Vector-Norm]{
    \br{\A_1, \sigma} \rightarrow \br{\N_1(n_1, 1), \sigma} \and
    \br{\A_2, \sigma} \rightarrow \br{\N_2(n_2, 1), \sigma} \and
    n_1 = n_2
    \\
    \br{\N_1(n_1, 1).\top \bmm \N_2(n_2, 1), \sigma} \rightarrow \br{\N(1, 1), \sigma}
  }{
    \br{\norm(\A_1, \A_2), \sigma} \rightarrow \br{\N(1, 1), \sigma}
  }
  \\
  \inferrule*[Right=Array-to-Real]{
    \n = \N(1,1)[0,0]
  }{
    \br{\N(1,1), \sigma} \rightarrow \br{\n, \sigma}
  }
  \\
  \inferrule*[Right=Power]{
    \n = \n_1^{\n_2}
  }{
    \br{\pow(\n_1, \n_2), \sigma} \rightarrow \br{\n, \sigma}
  }
  \and
  \inferrule*[Right=Square Root]{
    \n' = \sqrt{n}
  }{
    \br{\sqrtt(\n), \sigma} \rightarrow \br{\n', \sigma}
  }
\end{mathpar}

\subsection{Translation}
In our target language, we assume a grid layout for 2-dimensional arrays.
For each array $\A^{i}(n_i, m_i)$ in a program, a block shape $(\c^{i}_1, \c^{i}_2)$ is 
chosen. The block shape is comprised of two integers corresponding to 
the block's length along each axis of $\A^{i}(n_i, m_i)$ with the constraint that
if $n_i = n_j$ then $c^i_1 = c^j_1$ and if $m_i = m_j$ then $c^i_2 = c^j_2$.
Let $n//k$ be the integer division of $n$ by $k$. Then $\divup(n, k) = (n + k - 1) // k$ is the integer division of $n$ by $k$ rounded up.
For each array, we have a grid of $\divup(n, \c_1) \times \divup(m, \c_2)$ blocks.
We denote the 2-dimensional grid layout of array $\A^{i}$ by $\kappa^{i}_1 \times \kappa^{i}_2$. We drop the superscripts $i$ when the array in question is obvious.
An additional object id structure is given below to represent futures
for arrays. Below, we denote the object ids corresponding to blocks of an array
by $\o_{i, j}$ for $1 \leq i \leq \kappa_1 \wedge 1 \leq j \leq \kappa_2$.
\begin{align}
\o(\kappa_1, \kappa_2) & =
\begin{bmatrix}
    \o_{1, 1} & \dots & \o_{1, \kappa_2}  \\
    \vdots & \ddots & \vdots \\
     \o_{\kappa_1, 1} & \dots & \o_{\kappa_1, \kappa_2}
 \end{bmatrix}
\end{align}
We extend the syntax of object ids below to include the above data structure.
\begin{verbatim}
o ::= ... | o(\kappa_1, \kappa_2)
\end{verbatim}
The index set corresponding to the indices 
of the $i, j$ block of $\A$ is given by
$$\I(\kappa_1, \kappa_2)_{i,j} = \{ (i', j') \mid i' = (i-1)\c_1, \dots, i \c_1 - 1 \, ; \, j' = (j-1)\c_2, \dots, j \c_2 - 1 \}.$$
We assume for simplicity that the size of the last block along the first and second axes are $\min(\kappa_1 \c_1, n)$, and $\min(\kappa_2 \c_2, m)$, respectively.
Translations for arrays and their operators are defined as follows.

\subsubsection{Declaration}
\begin{align*}
\T(\Zeros(n, m)) & \equiv 
\begin{bmatrix}
    \R(\Zeros)(n, m, 1, 1) & \dots & \R(\Zeros)(n, m, 1, \kappa_2) \\
    \vdots & \ddots & \vdots \\
    \R(\Zeros)(n, m, \kappa_1, 1) & \dots & \R(\Zeros)(n, m, \kappa_1, \kappa_2) \\
\end{bmatrix}
\\
\T(\Read(\s, n, m)) & \equiv 
\begin{bmatrix}
    \R(\Read)(\s, n, m, 1, 1) & \dots & \R(\Read)(\s, n, m, 1, \kappa_2) \\
    \vdots & \ddots & \vdots \\
    \R(\Read)(\s, n, m, \kappa_1, 1) & \dots & \R(\Read)(\s, n, m, \kappa_1, \kappa_2) \\
\end{bmatrix}
\end{align*}

For brevity, we extend $\Zeros$ and $\Read$ in their remote counterparts to take
block indices.

\subsubsection{Selection}

Let $n', m'$ denote the dimensions of the array $\A'$ from which 
entries are being selected, and $n, m$ be the dimensions of the resulting array $\A$.
We denote by $\o'$ and $\o$ the object id to which $\A'$ and $\A$ are translated, respectively.
We know $n = i_2 - i_1$, $m = j_2 - j_1$, and 
we also denote by $\kappa_1', \kappa_2'$ the number of blocks in $\A'$,
and $\kappa_1, \kappa_2$ the number of blocks in $\A$.
We can now derive the index sets $\I'(\kappa_1', \kappa_2')_{i',j'}$ for the block representation
of $\A'$ and $\I(\kappa_1, \kappa_2)_{i,j}$ for the block representation of
$\A = \A'[i_1:i_2, j_1:j_2]$.
We define the selection set $\S_{i,j} = \{ (i_1 + i'', j_1 + j'' \mid (i'', j'') \in \I(\tau_1, \tau_2)_{i,j} \}$ to obtain $\args_{i, j} = \{ (i', j', o'_{i', j'}) \mid \I'(\kappa_1', \kappa_2')_{i',j'} \cap \S_{i, j} \neq \emptyset \},$ the arguments provided to
the operator $\Select(\args, i, j)$, where 
$\args = (\args_{i,j}, i_1, i_2, j_1, j_2)$. The selection operator
returns an object id $\o(\kappa_1, \kappa_2)_{i, j}$ corresponding to block $i,j$ of $\A = \A'[i_1:i_2, j_1:j_2]$. 

\begin{align*}
\T(\o'(\kappa_1', \kappa_2')[i_1:i_2, j_1:j_2]) & \equiv 
\begin{bmatrix}
    \R(\Select)(\args, 1, 1) & \dots & \R(\Select)(\args, 1, \kappa_2) \\
    \vdots & \ddots & \vdots \\
    \R(\Select)(\args, \kappa_1, 1) & \dots & \R(\Select)(\args, \kappa_1, \kappa_2)
\end{bmatrix}
\\
\T(\A'[i_1:i_2, j_1:j_2]) & \equiv \T(\T(x)[i_1:i_2, j_1:j_2])
\\
\T(\A'[i', :]) & \equiv \T(\A'[i':i'+1, 0:m'])
\\
\T(\A'[:, j']) & \equiv \T(\A'[0:n', j':j'+1])
\\
\T(\A'[i', j']) & \equiv \T(\A'[i':i'+1, j':j'+1])
\end{align*}

\subsubsection{Assignment}
Let $n', m'$ be the dimensions of $\A'$, the array to which new values are being assigned,
and $n'' = i_2 - i_1, m'' = j_2-j_1$ the dimensions of the array $\A''$ containing
the new values. We further define $\o'(m', n')$ and $\o''(m'', n'')$ as the object ids
corresponding to $\A'$ and $\A''$, respectively.
The number of blocks in $\A'$ and $\A''$ are $\kappa_1', \kappa_2'$ and $\kappa_1'', \kappa_2''$,
respectively.
We use $\Assign(\args, i, j)$, where $\args = (\args_{i,j}, \o''(\kappa_1'', \kappa_2'')_{i, j}, i_1, i_2, j_1, j_2)$, to denote the assignment $\A'[i_1:i_2, \, j_1:j_2]_{i, j} = \A''_{i, j}$.
We compute $\args_{i,j}$ in a similar fashion to what is done for the selection operator.
\begin{align*}
\o'(n', m')[i_1:i_2, \, j_1:j_2] = \o''(n'', m'') & \equiv 
\o'(n', m') = \begin{bmatrix}
    \R(\Assign)(\args, 1, 1) & \dots & \R(\Assign)(\args, 1, \kappa_2') \\
    \vdots & \ddots & \vdots \\
    \R(\Assign)(\args, \kappa_1', 1) & \dots & \R(\Assign)(\args, \kappa_1', \kappa_2') \\
\end{bmatrix}
\\
\x[i_1:i_2, \, j_1:j_2] = \e & \equiv \T(\T(\x)[i_1:i_2, \, j_1:j_2]) = \T(\e) 
\\
\x[i', :] = \e & \equiv \T(\T(\x)[i':i'+1, 0:m']) = \T(\e)
\\
\x[:, j'] = \e & \equiv \T(\T(\x)[0:n', j':j'+1]) = \T(\e)
\\
\x[i', j'] = \e & \equiv \T(\T(\x)[i':i'+1, j':j'+1]) = \T(\e)
\end{align*}
The $\Assign$ operator updates the entries of $\A'$ in block $i,j$ which intersect
the selection operator $[i_1:i_2, \, j_1:j_2]$. The resulting updated block is returned.
If a block has no intersection with the selection operator, then the unchanged object id corresponding to that block is returned.

\subsubsection{Operators}
We denote by $\x_1, \N_1(n_1, m_1), \o_1(n_1, m_1)$
the operands corresponding to the left-hand side of the $\mm$ operation,
and by $\x_2, \N_2(n_2, m_2), \o_2(n_2, m_2)$ the right-hand side.
The result is denoted by $\N(n, m)$ and $\o(n, m)$, where $n=n_1$ and $m=m_2$.
We use the notation $\o_1(n_1, m_1)_{i, :}$ and $\o_1(n_1, m_1)_{:, j}$
to correspond to the $i$th "row block" and $j$th "column block" of $\o_1$, respectively.
The remote function $\R(\mm)(\args_{i,j})$ computes the $i,j$ block of
the result $\N(n, m)$, where $\args_{i,j} = (\o_1(n_1, m_1)_{i, :}, \o_2(n_2, m_2)_{:, j}, i, j)$.
In short, the $\R(\mm)$ operator computes the 
result of the operation $\N_1(n_1, m_1)_{i,:} \bmm \N_2(n_2, m_2){:, j}$,
which corresponds to block $i, j$ of $\N(n, m)$.

For binary array operations, 
$\R(\bop)(\o^1_{i,j}, \o^1_{i,j}, i, j)$ denotes the parallel application of 
$\bop$ on block $i,j$ of $\o_1(n_1, m_1)$ and $\o_2(n_2, m_2)$;
% we use $\o_1$ to indicate $\o_1(n_1, m_1)$, $\o_2$ to indicate $\o_2(n_2, m_2)$.

For binary array-scalar operations, 
$\R(\bop)(\o^1_{i,j}, \o, i, j)$ denotes the parallel application of 
$\bop$ on block $i,j$ of $\o_1(n_1, m_1)$,
% where $\o_1$ corresponds to $\o_1(n_1, m_1)$, and 
$\o$ corresponds to the scalar $\n$.

Unary operations, such as $\x.\top$, are applied in parallel in the obvious way
and are ranged over with the notation $\Unary$.

\begin{align*}
\T(\o_1(n_1, m_1) \mm \o_2(n_2, m_2)) & \equiv 
\begin{bmatrix}
    \R(\mm)(\args_{1,1}) & \dots & \R(\mm)(\args_{1, \kappa_2}) \\
    \vdots & \ddots & \vdots \\
    \R(\mm)(\args_{\kappa_1, 1}) & \dots & \R(\mm)(\args_{\kappa_1,\kappa_2})
\end{bmatrix}
\\
\T(\x_1 \mm \x_2) & \equiv \T(\T(\x_1) \mm \T(\x_2))
\\
\T(\o_1(n_1, m_1) \bop \o_2(n_2, m_2)) & \equiv 
\begin{bmatrix}
    \R(\bop)(\o_1, \o_2, 1, 1) & \dots & \R(\bop)(\o_1, \o_2, 1, \kappa_2) \\
    \vdots & \ddots & \vdots \\
    \R(\bop)(\o_1, \o_2, \kappa_1,1) & \dots & \R(\bop)(\o_1, \o_2, \kappa_1,\kappa_2)
\end{bmatrix}
\\
\T(\o_1(n_1, m_1) \bop \o) & \equiv 
\begin{bmatrix}
    \R(\bop)(\o_1, \o, 1, 1) & \dots & \R(\bop)(\o_1, \o, 1, \kappa_2) \\
    \vdots & \ddots & \vdots \\
    \R(\bop)(\o_1, \o, \kappa_1,1) & \dots & \R(\bop)(\o_1, \o, \kappa_1,\kappa_2)
\end{bmatrix}
\\
\T(\x_1 \bop \x_2) & \equiv \T(\T(\x_1) \bop \T(\x_2))
\\
\T(\Unary(\o(n, m))) & \equiv 
\begin{bmatrix}
    \R(\Unary)(\o(n, m)_{1,1}) & \dots & \R(\Unary)(\o(n, m)_{1,\kappa_2}) \\
    \vdots & \ddots & \vdots \\
    \R(\Unary)(\o(n, m)_{\kappa_1,1}) & \dots & \R(\Unary)(\o(n, m)_{\kappa_1, \kappa_2})
\end{bmatrix}
\\
\T(\Unary(\x)) & \equiv \T(\Unary(\T(\x)))
\end{align*}

\subsubsection{Additional Array and Arithmetic Expressions}
\begin{align*}
\T(\pow(\x_1, \x_2)) & \equiv \R(\pow)(\T(\x_1), \T(\x_2)) \\
\T(\sqrtt(\x)) & \equiv \R(\sqrtt)(\T(\x)) \\
\T(\norm(\x_1, \x_2)) & \equiv \T(\sqrtt(\T(\x.\top \mm \x))) \\
\T(\o) & \equiv \o
\end{align*}

\subsection{Proof Of Correctness}

Our proof of correction for arrays follows trivially from our existing proof
of correctness for expressions. Consider the case where block shape and array
shape are $(1,1)$. Our proof of correctness for $n$-ary operations covers this
case. Recall the proof of $n$-ary operations follows from the proof 
for arbitrary functions. If an array $A$ has shape 
equivalent to its block shape (one large block), then its proof
of correctness is covered by our proof of correctness for arbitrary functions.
Now consider the case for arbitrary array sizes with arbitrary block shape.
The expressions that comprise each block in the translated 
arrays are each covered in our proof of theorem \ref{maintheorem}.
The proof is by induction on the translations of operations 
for 2-dimensional arrays. The proof approach follows 
the same process as the other proofs of correctness.

% \subsubsection{N-Dimensional Arrays}

% All but matrix multiplication trivially extend to n-dimensions.
% We need to show that our translation approach generalizes
% to the \verb|tensordot| operation.
