# Supplementary material for: NumS: Scalable Array Programming for the Cloud
Source: arXiv:2206.14276 source file (2022-07-13)
Supplement: Supplementary file 8 [file 010-notation.tex]

\section{Notation}

\begin{enumerate}
    \item Expressions $\e \in \mathcal{E}$
    \item Commands $\c \in \mathcal{C}$
    \item Program states $\sigma \in \Sigma$
    \item Program transitions $\rightarrow \subseteq ((\mathcal{E} \cup \mathcal{C}) \times \Sigma) \times ((\mathcal{E} \cup \mathcal{C}) \times \Sigma)$
    \item $\dots$
\end{enumerate}
