# Supplementary material for: NumS: Scalable Array Programming for the Cloud
Source: arXiv:2206.14276 source file (2022-07-13)
Supplement: Supplementary file 9 [file 070-experiments.tex]

\section{Experiments}
\label{appendix:evaluation}
% Anything we can't fit into the main manuscript can go here, if it's important.
